# Supplementary material for: Estimating the effect of joint interventions from observational data in sparse high-dimensional settings
Source: arXiv:1407.2451 ancillary file (2016-03-10)
Supplement: Supplementary file 1 [file supplement.pdf]

*Submitted to the Annals of Statistics*

# SUPPLEMENT TO "ESTIMATING THE EFFECT OF JOINT INTERVENTIONS FROM OBSERVATIONAL DATA IN SPARSE HIGH-DIMENSIONAL SETTINGS"

BY PREETAM NANDY, MARLOES H. MAATHUIS AND THOMAS S. RICHARDSON

This document contains supplementary information to the paper "Estimating the effect of joint interventions from observational data in sparse high-dimensional settings" [14]. We refer to [14] as the "main text".

**1. Markov equivalence class of DAGs.** A DAG encodes conditional independence relationships via the notion of *d-separation* ([15], Theorem 1.2.4, page 18). In general, several DAGs can encode the same conditional independence relationships and such DAGs form a *Markov equivalence class*. Two DAGs belong to the same Markov equivalence class if and only if they have the same skeleton and the same v-structures [23]. A Markov equivalence class of DAGs can be uniquely represented by a *completed partially directed acyclic graph* (CPDAG) [20], which is a graph that can contain both directed and undirected edges. Figure 2 of the main text shows an example of a CPDAG, as well as the DAGs in its Markov equivalence class. A CPDAG satisfies the following: $i \to j$ in the CPDAG if $i \to j$ in every DAG in the Markov equivalence class, and $i - j$ in the CPDAG if the Markov equivalence class contains a DAG for which $i \to j$ and a DAG for which $i \leftarrow j$. CPDAGs can be estimated from observational data using various algorithms [2, 20, 21]. The PC-algorithm [20] is one such algorithm (see Section 12), and has been shown to be consistent in certain sparse high-dimensional settings [4, 6, 8].

**2. A schematic representation of IDA.**

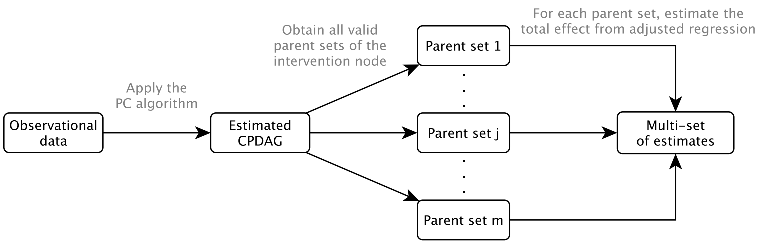


Fig 1: A schematic representation of the IDA algorithm.

**3. Single intervention effects as regression coefficients.** Let $\mathbf{X} = \{X_1, \dots, X_p\}$ be generated from a linear SEM characterized by $(\mathcal{G}, \boldsymbol{\epsilon})$. Our goal is to prove that if $X_p \notin \mathbf{PA}_1$ then the total effect of $X_1$ on $X_p$, denoted as $\theta_{1p}$, is equal to the regression coefficient of $X_1$ in the regression of $X_p$ on $X_1$ and $\mathbf{PA}_1$, denoted as $\beta_{1p|\mathbf{PA}_1}$ (Proposition 3.1). If the error variables are normally distributed, the proof of this result is straightforward and well known (e.g., [11]), since $\mathrm{E}[X_p|x_1, \mathbf{pa}_1]$ is a linear function of $x_1$ and $\mathbf{pa}_1$. The latter does not hold if we drop the normality assumption. However, we argue below that since both $\theta_{1p}$ and $\beta_{1p|\mathbf{PA}_1}$ depend on the distribution of $\mathbf{X}$ only through its covariance matrix (thanks to the linearity assumption), it suffices to prove the result assuming normally distributed errors.

PROPOSITION 3.1. *Let $\mathbf{X} = \{X_1, \dots, X_p\}$ be generated from a linear SEM characterized by $(\mathcal{G}, \boldsymbol{\epsilon})$. Then the total effect of $X_1$ on $X_p$, which is defined as $\theta_{1p} := \frac{\partial}{\partial x_1}\mathrm{E}[X_p|do(X_1 = x_1)]$, is equal to $\beta_{1p|\mathbf{PA}_1}$ if $X_p \notin \mathbf{PA}_1$ and is equal to zero if $X_p \in \mathbf{PA}_1$.*

PROOF. We first show that $\theta_{1p} = \beta_{1p|\mathbf{PA}_1}$ for a linear SEM with Gaussian noise. From Pearl's back-door adjustment [16], we have

$$f(x_p|do(X_1 = x_1)) = \begin{cases} \int f(x_p|x_1, \mathbf{pa}_1) f(\mathbf{pa}_1) d\mathbf{pa}_1 & \text{if } X_p \notin \mathbf{PA}_1 \\ f(x_p) & \text{otherwise,} \end{cases}$$

where we use $\mathbf{PA}_1$ as the adjustment set. Clearly, the total effect of $X_1$ on $X_p$ is zero if $X_p \in \mathbf{PA}_1$, while for $X_p \notin \mathbf{PA}_1$ we have

$$\mathrm{E}[X_p|do(X_1 = x_1)] = \int \mathrm{E}[X_p|x_1, \mathbf{pa}_1] f(\mathbf{pa}_1) d\mathbf{pa}_1.$$

Now if the error variables are normally distributed with $\mathrm{Cov}(\boldsymbol{\epsilon}) = D$ (or equivalently, the joint distribution of $\mathbf{X}$ is multivariate Gaussian), then $\mathrm{E}[X_p|x_1, \mathbf{pa}_1]$ is a linear function of $x_1$ and $\mathbf{pa}_1$ and hence $\theta_{1p} = \beta_{1p|\mathbf{PA}_1}$.

Let $B$ be the weight matrix of the weighted DAG $\mathcal{G}$, $D = \mathrm{Cov}(\boldsymbol{\epsilon})$ and $\Sigma = \mathrm{Cov}(\mathbf{X})$. Note that $\theta_{1p}$ can be computed from $B$ via the path method. We will show below that $B$ can be obtained uniquely from $\Sigma$, so that $\theta_{1p}$ only depends on the distribution of $X$ via $\Sigma$. Similarly, $\beta_{1p|\mathbf{PA}_1}$ only depends on the distribution of $X$ via $\Sigma$. Hence, $\theta_{1p}$ and $\beta_{1p|\mathbf{PA}_1}$ are identical for all linear SEMs $(\mathcal{G}, \boldsymbol{\epsilon})$ with weight matrix $B$ and error covariance matrix $D$, and we have shown that they are equal when the errors are normally distributed. As a result, they must be equal for any error distribution with error covariance matrix $D$.

It is left to show that there is a one-to-one correspondence between $\Sigma$ and the pair $(B, D)$. Since $\mathbf{X}$ is generated from the linear SEM $(\mathcal{G}, \boldsymbol{\epsilon})$, $\mathbf{X} =$

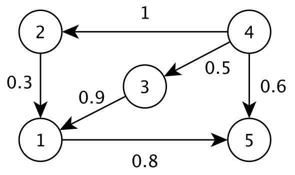


Fig 2: An example of a causal DAG where $\mathrm{E}[X_5|X_1 = x_1, \mathbf{PA}_1 = \mathbf{pa}_1]$ is a non-linear function of $\mathbf{pa}_1$ when the errors are i.i.d. Uniform$[-1, 1]$. (See Example 1.)

$(\mathrm{I} - B^T)^{-1}\boldsymbol{\epsilon}$ and hence $\Sigma = (\mathrm{I} - B^T)^{-1}D(\mathrm{I} - B^T)^{-T}$. When the vertices of $\mathcal{G}$ are ordered according to a causal order, then the weight matrix $B$ is upper triangular. Moreover, if $B$ is upper triangular, then $(\mathrm{I} - B^T)\Sigma(\mathrm{I} - B^T)^T = D$ represents the unique generalized Cholesky decomposition of $\Sigma$. Thus $(B, D)$ can be obtained (uniquely) from $\Sigma$, by rearranging rows and columns in $\Sigma$ according to a causal ordering for $\mathcal{G}$, and then computing its generalized Cholesky decomposition.

□

REMARK 3.1. *Let $\mathbf{BD}_1$ satisfy Pearl's backdoor criterion [16] relative to $X_1$ and $\mathbf{Y}$. By replacing $\mathbf{PA}_1$ by $\mathbf{BD}_1$ in the proof of Proposition 3.1, it then follows that $\theta_{1p} = \beta_{1p|\mathbf{BD}_1}$. For example, if there is no path from $X_1$ to $X_p$ that starts with an edge into $X_1$, then the empty set satisfies Pearl's backdoor criterion, and hence $\theta_{1p} = \beta_{1p|\emptyset}$.*

In the proof of Proposition 3.1, we used the fact that $\mathrm{E}[X_p|x_1, \mathbf{pa}_1]$ is a linear function of $x_1$ and $\mathbf{pa}_1$ when the error variables are normally distributed. For non-Gaussian errors, $\mathrm{E}[X_p|x_1, \mathbf{pa}_1]$ is linear in $x_1$ but can be non-linear in $\mathbf{pa}_1$. We illustrate this in the following example.

EXAMPLE 1. *Let $X_1, \ldots, X_5$ be generated from the linear SEM characterized by $(\mathcal{G}, \boldsymbol{\epsilon})$ with $\mathcal{G} = (\mathbf{V}, \mathbf{E}, B)$ depicted in Figure 2 and $\epsilon_1, \ldots, \epsilon_5 \overset{i.i.d.}{\sim}$* Uniform$[-1, 1]$. *Note that $\mathbf{PA}_1 = \{X_2, X_3\}$ and that the total effect of $X_1$ on $X_5$ is $\theta_{15} = 0.8$. We show that $\mathrm{E}[X_5|x_1, x_2, x_3] = 0.8x_1 + g(x_2, x_3)$, where $g(.)$ is a non-linear function of $x_2$ and $x_3$. We have:*

$$
\begin{aligned}
\mathrm{E}[X_5|x_1,x_2,x_3] &= \int_{-1}^{1} \mathrm{E}[X_5|x_1,x_2,x_3,x_4] f(x_4|x_1,x_2,x_3)\ dx_4 \\
&= \int_{-1}^{1} \mathrm{E}[X_5|x_1,x_4] f(x_4|x_2,x_3)\ dx_4 \\
&= 0.8x_1 \int_{-1}^{1} f(x_4|x_2,x_3)\ dx_4 + 0.6 \int_{-1}^{1} x_4 f(x_4|x_2,x_3)\ dx_4 \\
&= 0.8x_1 + 0.6\mathrm{E}[X_4|x_2,x_3],
\end{aligned}
$$

*where we used that $X_5$ is conditionally independent of its non-descendants $\{X_2, X_3\}$ given its parents $\{X_1, X_4\}$, and $X_1$ is conditionally independent of its non-descendant $X_4$ given its parents $\{X_2, X_3\}$.*

*Finally, we show that $\mathrm{E}[X_4|x_2,x_3]$ is a non-linear function of $x_2$ and $x_3$. The joint distribution of $X_2$, $X_3$ and $X_4$ is given by*

$$
f(x_2,x_3,x_4) = \begin{cases} 1/8 & \text{if } x_2 \in (x_4-1, x_4+1),\ x_3 \in (0.5x_4-1, 0.5x_4+1), \\ & \quad \text{and } x_4 \in (-1,1) \\ 0 & \text{otherwise} \end{cases} .
$$

*Therefore, for $x_2 \in (-2,2)$ and $x_3 \in (-1.5,1.5)$ such that $-3 < 2x_3 - x_2 < 3$, the conditional distribution of $X_4$ given $X_2 = x_2$ and $X_3 = x_3$ is* $\mathrm{Uniform}[a(x_2,x_3), b(x_2,x_3)]$*, where $a(x_2,x_3) = \max\{x_2-1, 2(x_3-1), -1\}$ and $b(x_2,x_3) = \min\{x_2+1, 2(x_3+1), 1\}$. Thus $\mathrm{E}[X_4|x_2,x_3] = (a(x_2,x_3) + b(x_2,x_3))/2$ is indeed a non-linear function of $x_2$ and $x_3$, since for example* $\mathrm{E}[X_4|0.5,-1] = -1/4$, $\mathrm{E}[X_4|0.5,0] = 1/4$ *and* $\mathrm{E}[X_4|0.5,1] = 1/2$.

## 4. Proofs of Section 3 of the main text.

**Proof of Theorem 3.1 of the main text.** We only consider the expression for $\theta_{1p}^{(1,2)}$. Suppose first that $X_2$ is a descendant of $X_1$ and $X_p$ is a descendant of $X_2$. Then $\theta_{1p}$ represents the effect of $X_1$ on $X_p$ along all directed paths from $X_1$ to $X_p$ and $\theta_{12}\theta_{2p}$ represents the effect of $X_1$ on $X_p$ along all directed paths that pass through $X_2$. Hence, correctness of the expression follows directly from the path method.

Next, suppose that $X_2$ is not a descendant of $X_1$ or $X_p$ is not a descendant of $X_2$. Then $\theta_{12}\theta_{2p} = 0$, so that $\theta_{1p}^{(1,2)} = \theta_{1p}$. This is again correct by the path method, since there are no directed paths from $X_1$ to $X_p$ that pass through $X_2$. □

**Proof of Theorem 3.2 of the main text.** Without loss of generality we assume that $i = 1$ and $j = k$. Thus, we need to prove that

$$
\theta_{1p}^{[k]}(\mathcal{G}) = \theta_{1p}^{[k-1]}(\mathcal{G}) - \theta_{1k}^{[k-1]}(\mathcal{G})\theta_{kp}^{[k]\setminus\{1\}}(\mathcal{G}), \tag{1}
$$

where we denote the dependence on $\mathcal{G}$ explicitly.

Let $\mathcal{G}'$ be the causal weighted DAG obtained from $\mathcal{G}$ by deleting all edges into nodes $2, \ldots, k-1$. Using the path method, all quantities in (1) can be computed from directed weighted paths in $\mathcal{G}$ that do not pass through $2, \ldots, k-1$. By construction, all such paths are identical in $\mathcal{G}$ and $\mathcal{G}'$. Hence, it is enough to prove (1) when we replace $\mathcal{G}$ by $\mathcal{G}'$.

Moreover, $\theta_{1p}^{[k]}(\mathcal{G}') = \theta_{1p}^{(1,k)}(\mathcal{G}')$, since there are no paths in $\mathcal{G}'$ that pass through nodes $2, \ldots, k-1$. Hence,

$$\begin{aligned}\theta_{1p}^{[k]}(\mathcal{G}') = \theta_{1p}^{(1,k)}(\mathcal{G}') &= \theta_{1p}(\mathcal{G}') - \theta_{1k}(\mathcal{G}')\theta_{kp}(\mathcal{G}') \\ &= \theta_{1p}^{[k-1]}(\mathcal{G}') - \theta_{1k}^{[k-1]}(\mathcal{G}')\theta_{kp}^{[k]\setminus\{i\}}(\mathcal{G}'),\end{aligned}$$

where the second equality follows from Theorem 3.1 of the main text and the last equality again follows from the definition of $\mathcal{G}'$. □

We need the following lemma to prove Theorem 3.3 of the main text. Note that we assume Gaussian error variables in Lemma 4.1. This is sufficient for the proof of Theorem 3.3, since both $\Sigma_k$ and $\Sigma^{[k]}$ depend on the distribution of $\mathbf{X}$ only through the covariance matrix $\Sigma$ (as in the proof of Proposition 3.1).

Lemma 4.1. *Let $\mathbf{X}$ be generated from a linear SEM $(\mathcal{G}, \boldsymbol{\epsilon})$ where the error variables are normally distributed. Let $j \neq i$, $|\mathbf{PA}_i| \geq 1$, $X_j \notin \mathbf{PA}_i$ and $\mathbf{W} \subseteq \mathbf{X} \setminus \{X_i, X_j\} \cup \mathbf{PA}_i$. Then the regression coefficients and the expected squared error in the regression $X_j \sim \mathbf{PA}_i + X_i + \mathbf{W}$, do not depend on the weights of the edges into vertex $i$ in the weighted DAG $\mathcal{G} = (\mathbf{V}, \mathbf{E}, B)$.*

Proof. Let $\mathbf{W}' = \{X_i\} \cup \mathbf{PA}_i \cup \mathbf{W}$. Since the distribution of $\mathbf{X}$ is multivariate Gaussian, $\mathrm{E}[X_j|\mathbf{W}' = \mathbf{w}'] = \boldsymbol{\beta}^T\mathbf{w}'$ where $\boldsymbol{\beta}$ is the vector of regression coefficients. Moreover, $\mathrm{Var}[X_j|\mathbf{W}' = \mathbf{w}']$ does not depend on $\mathbf{w}'$ and is equal to the expected squared error in the regression $X_j \sim \mathbf{W}'$. Therefore, it is sufficient to show that the conditional distribution of $X_j$ given $\mathbf{W}'$ does not depend on the weights of the edges into vertex $i$.

Recall that the joint density $f(x_1, \ldots, x_p)$ factorizes as $\prod_{r=1}^p f(x_r|\mathbf{pa}_r)$, where each $f(x_r|\mathbf{pa}_r)$ depends only on those edge weights that correspond to edges into vertex $r$ in $\mathcal{G}$. Therefore, $f(x_1, \ldots, x_p)/f(x_i|\mathbf{pa}_i) = \prod_{r\neq i} f(x_r|\mathbf{pa}_r)$ does not depend on the weights of the edges into vertex $i$ in $\mathcal{G}$. Moreover, the distribution of $\mathbf{PA}_i$ also does not depend on edges into vertex $i$. Thus $f(x_1, \ldots, x_p|x_i, \mathbf{pa}_i) = f(x_1, \ldots, x_p)/(f(x_i|\mathbf{pa}_i)f(\mathbf{pa}_i))$ does not depend on the weights of the edges into vertex $i$. This completes the proof, since $f(x_j|\mathbf{w}') = f(x_j|x_i, \mathbf{pa}_i, \mathbf{w}) = f(x_j, \mathbf{w}|x_i, \mathbf{pa}_i)/f(\mathbf{w}|x_i, \mathbf{pa}_i)$. □

**Proof of Theorem 3.3 of the main text.** As in the proof of Proposition 3.1, it suffices to prove the result assuming that the joint distribution of $\mathbf{X}$ is multivariate Gaussian (i.e., error variables are normally distributed) with covariance $\Sigma$, since both $\Sigma_k$ and $\Sigma^{[k]}$ are functions of the covariance matrix $\Sigma$. Thus, in the rest of the proof we assume that $\mathbf{X}$ is generated from a linear SEM $(\mathcal{G}, \boldsymbol{\epsilon})$ where the error variables are normally distributed.

Since Algorithm 3.1 of the main text is an iterative procedure, it is sufficient to prove the theorem for $k = 1$. Thus, we will show below that the algorithm produces $\Sigma_1 := \mathrm{Cov}(\mathbf{X}')$ from $\Sigma$, where $\mathbf{X}' := (X_1', \ldots, X_p')$ is generated from $(\mathcal{G}_1, \boldsymbol{\epsilon})$. Recall that $\mathcal{G}_1$ is obtained from $\mathcal{G}$ by deleting all edges into vertex $i$. Thus if $\mathbf{PA}_1 = \emptyset$ then $\mathcal{G} = \mathcal{G}_1$ and hence $\Sigma = \Sigma_1$. In this case the algorithm also does not make any change to $\Sigma$. Hence, we assume that $q_1 := |\mathbf{PA}_1| \geq 1$.

Without loss of generality, we assume that the variables in $\Sigma$ (and similarly in $\Sigma_1$) are ordered as $X_{r_1}, \ldots, X_{r_p}$ where $\{X_{r_1}, \ldots, X_{r_{q_1}}\} = \mathbf{PA}_1$ and $X_{r_{q_1+1}} = X_1$. Let $L\Sigma L^T = D$ and $L'\Sigma_1 L'^T = D'$ be the Cholesky decompositions of $\Sigma$ and $\Sigma_1$. Then we complete the proof by showing that $D' = D$ and $L' = L$ except for the $(q_1 + 1)$th row which is equal to $\mathbf{e}_{q_1+1}^T$. Note that this implies that the algorithm produces $\Sigma_1$ from $\Sigma$.

Recall that by definition both $L'$ and $L$ are lower triangular matrices with $1's$ in the diagonals. For $j < i$, $-L_{ij}$ is the regression coefficients of $X_{r_j}$ in the regression $X_{r_i} \sim X_{r_1} + \cdots + X_{r_{i-1}}$ (see, for example, [17]) and similarly, $-L'_{ij}$ is the regression coefficients of $X'_{r_j}$ in the regression $X'_{r_i} \sim X'_{r_1} + \cdots + X'_{r_{i-1}}$. Since $\mathrm{E}[\mathbf{X}] = \mathbf{0}$ and $\mathrm{Cov}(L\mathbf{X}) = L\Sigma L^T = D$, for all $1 \leq i \leq q$ we have, $\mathrm{E}[X_{r_i} + \sum_{j=1}^{i-1} L_{ij} X_{r_j}]^2 = D_{ii}$ and similarly, $\mathrm{E}[X'_{r_i} + \sum_{j=1}^{i-1} L'_{ij} X'_{r_j}]^2 = D'_{ii}$.

For $i \leq q_1$, $L'_{ij} = L_{ij}$ and $D'_{ii} = D_{ii}$ follow from the fact that $(X_{r_1}, \ldots, X_{r_{q_1}})$ and $(X'_{r_1}, \ldots, X'_{r_{q_1}})$ are identically distributed since deletion of edges into vertex $i$ would only change the distribution of its descendants of $X_1$ (including $X_1$). The same holds for $i > q_1 + 1$ since the weight matrices of $\mathcal{G}$ and $\mathcal{G}_1'$ are identical except for the entries that correspond to the edges into vertex 1 and Lemma 4.1 (with $i = 1$, $j = r_i$ and $\mathbf{W} = \{X_{r_s} : s = q_1 + 2, \ldots, r_i - 1\}$) assures that the regression coefficients and the expected squared error in the regression $X_{r_i} \sim X_{r_1} + \ldots + X_{r_{i-1}}$ do not depend on the entries of the weight matrix that correspond to the edges into vertex 1.

Finally, for $i = q_1 + 1$, $X'_{r_i} = X'_1 = \epsilon_1$ and hence $X'_{r_i}$ is independent of $(X'_{r_1}, \ldots, X'_{r_{i-1}})$. Thus the $(q_1 + 1)$-th row of $L'$ is indeed equal to $\mathbf{e}_{q_1+1}^T$ and $D'_{ii} = \mathrm{E}[\epsilon_1^2]$. On the other hand, we have, $D_{ii} = \mathrm{E}[\epsilon_1^2]$ since $X_1 = \sum_{i=1}^{q_1} B_{r_i 1} X_i + \epsilon_1$, where $\epsilon_1$ is independent of $\{X_{r_1}, \ldots, X_{r_{q_1}}\}$. □

**Proof of Theorem 3.4 of the main text.** Let $\Sigma = \mathrm{Cov}(\mathbf{X})$ and $\Sigma_{\mathbf{U}} =$

Cov($\mathbf{U}$). Let $\Sigma^{[k]}$ and $(\Sigma_{\mathbf{U}})^{[k]}$ be the output of Algorithm 3.1 of the main text applied to $\Sigma$ and $\Sigma_{\mathbf{U}}$ respectively. Then it is sufficient to show that $(\Sigma_{\mathbf{U}})^{[k]} = (\Sigma^{[k]})_{\mathbf{U}}$, since $\theta_{ip}^{(1,\dots,k)}(\mathcal{G}) = (\Sigma_k)_{x_i x_p}/(\Sigma_k)_{x_i x_i}$ (where $\Sigma_k$ is defined in (5)) of the main text and Theorem 3.4 of the main text shows that $\Sigma^{[k]} = \Sigma_k$.

Now since Algorithm 3.1 of the main text is an iterative procedure, it is sufficient to prove $(\Sigma_{\mathbf{U}})^{[1]} = (\Sigma^{[1]})_{\mathbf{U}}$. Without loss of generality, assume that the first block of rows of $\Sigma$ (and $\Sigma^{[1]}$) correspond to $\mathbf{U}$. Let $(L_{\mathbf{U}}, D_{\mathbf{U}})$ be the unique generalized Cholesky decomposition of $\Sigma_{\mathbf{U}}$. Then $(\Sigma_{\mathbf{U}})^{[1]} = (\Sigma^{[1]})_{\mathbf{U}}$ follows from the fact the $L_{\mathbf{U}}$ and $D_{\mathbf{U}}$ are identical to the principal submatrices (that correspond to $\mathbf{U}$) of the lower triangular matrix $L$ and the diagonal matrix $D$ of the Cholesky decomposition of $\Sigma$. □

**Proof of Theorem 3.5 of the main text.** If $X_p \in \mathbf{PA}_1$ then $\hat{\theta}_{1p} = \tilde{\theta}_{1p} = 0$. Also note that the result trivially holds if $\mathbf{PA}_1 = \emptyset$. Thus we assume $\mathbf{PA}_1 = \{X_{r_1}, \dots, X_{r_{q_1}}\} \neq \emptyset$ and $X_p \notin \mathbf{PA}_1$. Let $\hat{\Sigma}$ be the sample covariance matrix of $\mathbf{U} = (X_{r_1}, \dots, X_{r_{q_1}}, X_1, X_p)^T$ and let $\hat{\Sigma}^{[1]}$ be the output of the Algorithm 3.1 of the main text applied to $\hat{\Sigma}$. Let $(L, D)$ be the Cholesky decomposition of $\hat{\Sigma}$ and let $\tilde{L}$ be the modification of $L$ produced by Algorithm 3.1 of the main text and thus $\tilde{L}\hat{\Sigma}^{[1]}\tilde{L}^T = D$.

Let $\mathcal{G}^*$ and $\tilde{\mathcal{G}}$ be the DAGs with weight matrices $B^* = \mathrm{I} - L$ and $\tilde{B} = \mathrm{I} - \tilde{L}$ respectively and the identical vertex set $\mathbf{V}^* = \{r_1, \dots, r_{q_1}, 1, p\}$. Let $\mathbf{Y}$ and $\tilde{\mathbf{Y}}$ be generated from the linear SEMs $(\mathcal{G}^*, \boldsymbol{\epsilon}^*)$ and $(\tilde{\mathcal{G}}, \boldsymbol{\epsilon}^*)$ respectively, where $\mathrm{Cov}(\boldsymbol{\epsilon}^*) = D$. Thus $\mathrm{Cov}(\mathbf{Y}^*) = \hat{\Sigma}$ and $\mathrm{Cov}(\tilde{\mathbf{Y}}) = \hat{\Sigma}^{[1]}$. On the other hand, since $\mathcal{G}^*$ and $\tilde{\mathcal{G}}$ are identical except for the edges into vertex 1, $\theta_{1p}(\mathcal{G}^*) = \theta_{1p}(\tilde{\mathcal{G}})$. This completes the proof since $\hat{\theta}_{1p} = \theta_{1p}(\mathcal{G}^*)$ and $\tilde{\theta}_{1p} = \theta_{1p}(\tilde{\mathcal{G}})$. □

## 5. RRC versus Cochran's recursion relation.

As noted after Theorem 3.1 of the main text, the RRC formula $\theta_{1p}^{(1,2)} = \theta_{1p} - \theta_{12}\theta_{2p}$ seems to resemble Cochran's recursion relation $\beta_{1p|2} = \beta_{1p} - \beta_{12}\beta_{2p|1}$ [3]. The main difference between these two formulas is that Cochran's formula contains regression coefficients, while RRC contains causal effects (which may or may not be the same as the regression coefficients in Cochran's formula). The following example shows that the formulas can be fully identical (Figure 3a) or fully different (Figure 3b). Moreover, it can also happen that the left hand sides of the formulas are equal, while the quantities on the right hand side are all different (Figure 3c).

EXAMPLE 2. *In this example, we point out similarities and differences between the RRC formula and Cochran's recursion relation.*

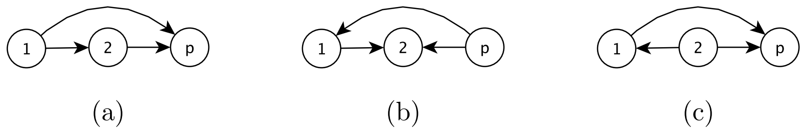


Fig 3: Examples of DAGs where (a) $\theta_{1p}^{(1,2)} = \beta_{1p|2}$, (b) $\theta_{1p}^{(1,2)} \neq \beta_{1p|2}$ and (c) $\theta_{1p} \neq \beta_{1p}$ but $\theta_{1p}^{(1,2)} = \beta_{1p|2}$. (See Example 2.)

*In Figure 3a, we have* $\theta_{1p} = \beta_{1p}$ *and* $\theta_{12} = \beta_{12}$*, since* $\mathbf{PA}_1 = \emptyset$ *satisfies the backdoor criterion. Moreover,* $\theta_{2p} = \beta_{2p|1}$ *since* $\mathbf{PA}_2 = \{1\}$*. Hence,* $\theta_{1p}^{(1,2)} = \beta_{1p|2}$.

*In Figure 3b, we have* $\theta_{1p}^{(1,2)} = 0$*, but* $\beta_{1p|2}$ *is in general nonzero. Moreover,* $\theta_{1p} = 0 \neq \beta_{1p}$, $\theta_{12} = \beta_{12|p} \neq \beta_{12}$ *and* $\theta_{2p} = 0 \neq \beta_{2p|1}$ *(except for very special choices of the edge weights).*

*In Figure 3c, we have* $\theta_{1p}^{(1,2)} = \theta_{1p} = \beta_{1p|2}$*, since* $\mathbf{PA}_1 = \{2\}$*. However,* $\theta_{1p} = \beta_{1p|2} \neq \beta_{1p}$, $\theta_{12} = 0 \neq \beta_{12}$ $\theta_{2p} = \beta_{2p} \neq \beta_{2p|1}$ *(except for very special choices of the edge weights).*

## 6. An illustration of the MCD algorithm.

EXAMPLE 3. *We reconsider Example 1 of the main text, where we assume that* $\mathbf{X} = (X_1, \ldots, X_6)$ *is generated from a linear SEM characterized by* $(\mathcal{G}, \boldsymbol{\epsilon})$ *with* $\mathcal{G}$ *given in Figure 1 of the main text and* $\mathrm{Cov}(\boldsymbol{\epsilon}) = \mathrm{I}$*. The weight matrix* $B$ *of the weighted DAG* $\mathcal{G}$ *is given by*

$$B = \begin{array}{c} \\ 1 \\ 2 \\ 3 \\ 4 \\ 5 \\ 6 \end{array} \begin{array}{c} \begin{array}{cccccc} 1 & 2 & 3 & 4 & 5 & 6 \end{array} \\ \begin{pmatrix} 0 & 0 & 1.1 & 0.3 & 0 & 0 \\ 0 & 0 & 0 & 0 & 0 & 0.4 \\ 0 & 0.6 & 0 & 0.8 & 0 & 0.9 \\ 0 & 0.5 & 0 & 0 & 0 & 0 \\ 0.2 & 0 & 0 & 0.7 & 0 & 0 \\ 0 & 0 & 0 & 0 & 0 & 0 \end{pmatrix} \end{array}.$$

*Hence,* $\Sigma = \mathrm{Cov}(\mathbf{X}) = (I - B^T)^{-1}\mathrm{Cov}(\boldsymbol{\epsilon})(I - B^T)^{-T} = (I - B^T)^{-1}(I -$

$B^T)^{-T}$, *which yields*

$$\Sigma = \begin{array}{c} \\ X_1 \\ X_2 \\ X_3 \\ X_4 \\ X_5 \\ X_6 \end{array} \begin{array}{c} \begin{array}{cccccc} X_1 & X_2 & X_3 & X_4 & X_5 & X_6 \end{array} \\ \begin{pmatrix} 1.04 & 1.37 & 1.14 & 1.37 & 0.20 & 1.58 \\ 1.37 & 4.17 & 2.51 & 3.34 & 0.60 & 3.93 \\ 1.14 & 2.51 & 2.26 & 2.30 & 0.22 & 3.04 \\ 1.37 & 3.34 & 2.30 & 3.91 & 0.94 & 3.41 \\ 0.20 & 0.60 & 0.22 & 0.94 & 1.00 & 0.44 \\ 1.58 & 3.93 & 3.04 & 3.41 & 0.44 & 5.30 \end{pmatrix} \end{array}.$$

*We now assume that we are* not *given $\mathcal{G}$ or $B$, but we are only given $\Sigma$ and the parent sets of $X_1$ and $X_2$, namely $\mathbf{PA}_1 = \{5\}$ and $\mathbf{PA}_2 = \{3, 4\}$. We will compute the total joint effect of $(X_1, X_2)$ on $X_6$ using the MCD algorithm. Note that $\mathbf{U} := \{X_1, X_2, X_6\} \cup \mathbf{PA}_1 \cup \mathbf{PA}_2 = \mathbf{X}$, and hence $\mathrm{Cov}(\mathbf{U}) = \Sigma$.*

*We follow the steps of the MCD oracle algorithm. First, we re-order the variables in $\Sigma^{[0]} = \Sigma$ as $(\mathbf{PA}_1, X_1, \mathbf{U} \setminus (\mathbf{PA}_1 \cup \{X_1\}))$. For example, we can choose the ordering $(X_5, X_1, X_2, X_3, X_4, X_6)$. Next, we obtain the Cholesky decomposition $L^{[0]}\Sigma^{[0]}(L^{[0]})^T = D^{[0]}$, where $D^{[0]}$ is a diagonal matrix with diagonal entries $\{1, 1, 2.25, 0.56, 0.8, 1\}$ and*

$$L^{[0]} = \begin{array}{c} \\ X_5 \\ X_1 \\ X_2 \\ X_3 \\ X_4 \\ X_6 \end{array} \begin{array}{c} \begin{array}{cccccc} X_5 & X_1 & X_2 & X_3 & X_4 & X_6 \end{array} \\ \begin{pmatrix} 1.00 & 0.00 & 0.00 & 0.00 & 0.00 & 0.00 \\ -0.20 & 1.00 & 0.00 & 0.00 & 0.00 & 0.00 \\ -0.35 & -1.25 & 1.00 & 0.00 & 0.00 & 0.00 \\ 0.16 & -0.54 & -0.44 & 1.00 & 0.00 & 0.00 \\ -0.56 & -0.24 & -0.40 & -0.40 & 1.00 & 0.00 \\ 0.00 & 0.00 & -0.40 & -0.90 & 0.00 & 1.00 \end{pmatrix} \end{array}.$$

*Note that the second row of $L^{[0]}$, i.e., the row corresponding to $X_1$, is identical to $(-B_{51}, 1, 0, 0, 0, 0)$.*

*Next, we replace the second row of $L^{[0]}$ by $(0, 1, 0, 0, 0, 0)$ to obtain $L^{(1)}$ and*

$$\Sigma^{[1]} = (L^{[1]})^{-1}D^{[0]}(L^{[1]})^{-T} = \begin{array}{c} \\ X_5 \\ X_1 \\ X_2 \\ X_3 \\ X_4 \\ X_6 \end{array} \begin{array}{c} \begin{array}{cccccc} X_5 & X_1 & X_2 & X_3 & X_4 & X_6 \end{array} \\ \begin{pmatrix} 1.00 & 0.00 & 0.35 & 0.00 & 0.70 & 0.14 \\ 0.00 & 1.00 & 1.25 & 1.10 & 1.18 & 1.49 \\ 0.35 & 1.25 & 3.93 & 2.37 & 3.02 & 3.71 \\ 0.00 & 1.10 & 2.37 & 2.21 & 2.10 & 2.94 \\ 0.70 & 1.18 & 3.02 & 2.10 & 3.52 & 3.10 \\ 0.14 & 1.49 & 3.71 & 2.94 & 3.10 & 5.13 \end{pmatrix} \end{array}.$$

*We then re-order the variables in $\Sigma^{[1]}$ as $(\mathbf{PA}_2, X_2, \mathbf{U} \setminus (\mathbf{PA}_2 \cup \{X_2\}))$. For example, we can choose $(X_3, X_4, X_2, X_1, X_5, X_6)$. We then repeat the*

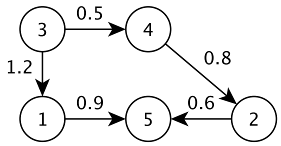


Fig 4: An example of a causal DAG where both MCD and RRC work for an incorrect specification of parent sets. (See Example 4.)

*procedure of computing the Cholesky decomposition* $L^{[1]}\Sigma^{[1]}(L^{[1]})^T = D^{[1]}$, *modifying* $L^{[1]}$ *to obtain* $L^{[2]}$, *and computing* $\Sigma^{[2]} = (L^{[2]})^{-1}D^{[1]}(L^{[2]})^{-T}$. *After re-ordering the variables in* $\Sigma^{[2]}$ *as* $(X_1, \dots, X_6)$ *we obtain*

$$\Sigma^{[2]} = \begin{array}{c} \\ X_1 \\ X_2 \\ X_3 \\ X_4 \\ X_5 \\ X_6 \end{array} \begin{array}{c} \begin{array}{cccccc} X_1 & X_2 & X_3 & X_4 & X_5 & X_6 \end{array} \\ \begin{pmatrix} 1.00 & 0.00 & 1.10 & 1.18 & 0.00 & 0.99 \\ 0.00 & 1.00 & 0.00 & 0.00 & 0.00 & 0.40 \\ 1.10 & 0.00 & 2.21 & 2.10 & 0.00 & 1.99 \\ 1.18 & 0.00 & 2.10 & 3.52 & 0.70 & 1.89 \\ 0.00 & 0.00 & 0.00 & 0.70 & 1.00 & 0.00 \\ 0.99 & 0.40 & 1.99 & 1.89 & 0.00 & 2.95 \end{pmatrix} \end{array}.$$

*This is the covariance matrix of* $\mathbf{X}$ *after intervening on* $X_1$ *and* $X_2$.

*Finally, we compute the total joint effect of* $(X_1, X_2)$ *on* $X_6$ *from* $\Sigma^{(1,2)}$:

$$(\theta_{16}^{(1,2)}, \theta_{26}^{(1,2)}) = \left(\frac{\Sigma_{16}^{[2]}}{\Sigma_{11}^{[2]}}, \frac{\Sigma_{26}^{[2]}}{\Sigma_{22}^{[2]}}\right)^T = (0.99, 0.4)^T.$$

*The result is identical to the result of the path method in Example 1 of the main text.*

## 7. MCD and RRC with incorrectly specified parent sets.

Example 4. *Let* $X_1, \dots, X_5$ *be generated from a linear SEM characterized by* $(\mathcal{G}, \boldsymbol{\epsilon})$, *where* $\mathcal{G} = (\mathbf{V}, \mathbf{E}, B)$ *is depicted in Figure 4 and* $\boldsymbol{\epsilon} = (\epsilon_1, \dots, \epsilon_5)^T$ *are jointly independent errors with arbitrary zero mean distributions. Note that* $\mathbf{PA}_1 = \{3\}$ *and* $\mathbf{PA}_2 = \{4\}$. *Since there is no directed path from* $X_1$ *to* $X_2$ *nor from* $X_2$ *to* $X_1$, $\theta_{15}^{(1,2)} = \theta_{15} = \beta_{15|3} = 0.9$ *and* $\theta_{25}^{(1,2)} = \theta_{25} = \beta_{25|4} = 0.6$.

*We define the following alternative "parent sets":* $\mathbf{PA}'_1 = \emptyset$ *and* $\mathbf{PA}'_2 = \{4\}$, *where* $\mathbf{PA}'_1 \neq \mathbf{PA}_1$. *Then the output of MCD (see Algorithm 3.2 of the*

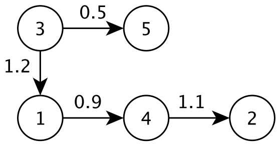


Fig 5: An example of a causal DAG where MCD works but RRC does not work for an incorrect specification of parent sets. (See Example 5.)

*main text) with parent sets* $\mathbf{PA}_1'$ *and* $\mathbf{PA}_2'$ *is still equal to* $(0.9, 0.6)^T$. *In this case, the MCD algorithm only sets the weight of the edge* $4 \to 2$ *to zero. But this is sufficient for computing the joint effects from (unadjusted) regressions (see line 2 of Algorithm 3.2), since after removing the edge* $4 \to 2$, *there is no backdoor path from node* $1$ *to node* $5$ *nor from node* $2$ *to node* $5$ *in the resulting graph.*

*If we apply RRC with parent sets* $\mathbf{PA}_1'$ *and* $\mathbf{PA}_2'$, *we get* $\theta_{15}^{(1,2)}(\mathbf{PA}_1', \mathbf{PA}_2') = \beta_{15} - \beta_{12}\beta_{25|4}$ *and* $\theta_{25}^{(1,2)}(\mathbf{PA}_1', \mathbf{PA}_2') = \beta_{25|4} - \beta_{21|4}\beta_{15}$. *The correct causal effects are given by* $\theta_{15}^{(1,2)}(\mathbf{PA}_1, \mathbf{PA}_2)$ *and* $\theta_{25}^{(1,2)}(\mathbf{PA}_1, \mathbf{PA}_2)$.

*We first show that* $\theta_{25}^{(1,2)}(\mathbf{PA}_1', \mathbf{PA}_2') = \theta_{25}^{(1,2)}(\mathbf{PA}_1, \mathbf{PA}_2)$. *Note that* $\beta_{21|4} = \theta_{21} = 0$, *since there is no directed path from node* $2$ *to node* $1$. *Therefore,* $\theta_{25}^{(1,2)}(\mathbf{PA}_1', \mathbf{PA}_2') = \beta_{25|4} = \theta_{25}^{(1,2)}(\mathbf{PA}_1, \mathbf{PA}_2)$. *Next, one can easily check (by computing regression coefficients) that* $\theta_{15}^{(1,2)}(\mathbf{PA}_1', \mathbf{PA}_2') = \beta_{15} - \beta_{12}\beta_{25|4} = \beta_{15|3} = \beta_{15|3} - \beta_{12|3}\beta_{25|4} = \theta_{15}^{(1,2)}(\mathbf{PA}_1, \mathbf{PA}_2)$ *(although* $\beta_{15} \neq \beta_{15|3}$ *and* $\beta_{12} \neq \beta_{12|3}$*).*

Example 5. *Let* $X_1, \ldots, X_5$ *be generated from a linear SEM characterized by* $(\mathcal{G}, \boldsymbol{\epsilon})$, *where* $\mathcal{G} = (\mathbf{V}, \mathbf{E}, B)$ *is depicted in Figure 5 and* $\boldsymbol{\epsilon} = (\epsilon_1, \ldots, \epsilon_5)^T$ *are jointly independent errors with arbitrary zero mean distributions. Note that* $\mathbf{PA}_1 = \{3\}$ *and* $\mathbf{PA}_2 = \{4\}$. *Since there is no directed path from* $X_1$ *to* $X_5$ *nor from* $X_2$ *to* $X_5$, $\theta_{15}^{(1,2)} = \theta_{25}^{(1,2)} = 0$.

*We define the following alternative "parent sets":* $\mathbf{PA}_1' = \{3\}$ *and* $\mathbf{PA}_2' = \emptyset$, *where* $\mathbf{PA}_2' \neq \mathbf{PA}_2$. *Then the output of MCD (see Algorithm 3.2 of the main text) with parent sets* $\mathbf{PA}_1'$ *and* $\mathbf{PA}_2'$ *is still equal to* $(0, 0)^T$, *since it is sufficient to remove the edge* $3 \to 1$ *for computing the joint effects from (unadjusted) regressions (see line 2 of Algorithm 3.2).*

*However, if we apply RRC with parent sets* $\mathbf{PA}_1'$ *and* $\mathbf{PA}_2'$, *we get*

$$\theta_{15}^{(1,2)}(\mathbf{PA}_1', \mathbf{PA}_2') = \beta_{15|3} - \beta_{12|3}\beta_{25} = -0.99\beta_{25} \neq 0.$$

*Note that* $\beta_{25}$ *is nonzero because* $X_2$ *and* $X_5$ *are marginally correlated, and the last equality follows from* $\beta_{15|3} = \theta_{15} = 0$ *and* $\beta_{12|3} = \theta_{12} = 0.99$.

*Moreover,* $\theta_{25}^{(1,2)}(\mathbf{PA}_1', \mathbf{PA}_2') \neq 0$*, since* $\theta_{25}^{(1,2)}(\mathbf{PA}_1', \mathbf{PA}_2') = \beta_{25} - \beta_{21}\beta_{15|3} = \beta_{25} \neq 0$.

## 8. Proofs of Section 4 of the main text.

**Proof of Theorem 4.1 of the main text.** Let $\hat{\boldsymbol{\theta}} := (\hat{\theta}_{1p}, \hat{\theta}_{2p}, \hat{\theta}_{12}, \hat{\theta}_{21})^T$. Since $X_j \notin \mathbf{PA}_i$, $\theta_{ij} = \beta_{ij|\mathbf{PA}_i}$ and $\hat{\theta}_{ij} = \hat{\beta}_{ij|\mathbf{PA}_i}$ for any $i \in \{1,2\}$, $j \in \{1,2,p\}$ and $i \neq j$. Hence, there is a differentiable function $h_1 : \mathbb{R}^{q(q+1)/2} \to \mathbb{R}^4$ such that $h_1(\mathrm{vech}(\Sigma)) = \boldsymbol{\theta}$ and $h_1(\mathrm{vech}(\hat{\Sigma})) = \hat{\boldsymbol{\theta}}$. Therefore, equation (8) of the main text and the multivariate delta-method imply

$$\sqrt{n}(\hat{\boldsymbol{\theta}} - \boldsymbol{\theta}) \xrightarrow{d} \mathcal{N}\left(\mathbf{0}, \Lambda\Gamma\Lambda^T\right).$$

The result now follows after applying the multivariate delta-method once again, since $h_2(\hat{\boldsymbol{\theta}}) = \hat{\boldsymbol{\theta}}_p^{(1,2)}$ and $h_2(\boldsymbol{\theta}) = \boldsymbol{\theta}_p^{(1,2)}$, where $h_2(x_1, x_2, x_3, x_4) = (x_1 - x_2x_3, x_2 - x_1x_4)^T$. □

In the following Proposition we derive an expression for $\Lambda$ given in Theorem 4.1 of the main text, which can be used to compute it explicitly (this was for example used for the computations in Section 9). We define $\mathbf{Z}_i := (\mathbf{PA}_i^T, X_i)^T$ and $q_i := |\mathbf{PA}_i|$ for $i = 1, \ldots, p$. For any $q \times q$ matrix $H$ and any sub-vectors $\mathbf{Z}$ and $\mathbf{W}$ of the $q \times 1$ vector $\mathbf{U}$, we let $H_{\mathbf{zw}}$ denote the sub-matrix of $H$ with rows and columns corresponding to $\mathbf{Z}$ and $\mathbf{W}$, respectively. We write $H_{\mathbf{zz}}^{-1}$ to denote $(H_{\mathbf{zz}})^{-1}$. Moreover, $\mathbf{e}_r$ denotes the $r$-th column of an identity matrix of appropriate dimension and $diag(A)$ denotes the diagonal matrix whose diagonal is identical to the diagonal of $A$.

PROPOSITION 8.1. *(Expression for $\Lambda$ in Theorem 4.1 of the main text) Assume that $\{X_1, X_2, X_p\} \cap (\mathbf{PA}_1 \cup \mathbf{PA}_2) = \emptyset$. Then*

$$\Lambda = \left[\mathrm{vech}\left(\frac{\partial\theta_{1p}}{\partial\Sigma}\right), \mathrm{vech}\left(\frac{\partial\theta_{2p}}{\partial\Sigma}\right), \mathrm{vech}\left(\frac{\partial\theta_{12}}{\partial\Sigma}\right), \mathrm{vech}\left(\frac{\partial\theta_{21}}{\partial\Sigma}\right)\right]^T,$$

*where for any $i \in \{1,2\}$, $j \in \{1,2,p\}$ and $i \neq j$, the $q \times q$ symmetric matrix $\frac{\partial\theta_{ij}}{\partial\Sigma}$ satisfies:*

*(i)* $\frac{\partial\theta_{ij}}{\partial\Sigma_{\mathbf{z}_i\mathbf{z}_i}} = -\left[H^{(ij)} + H^{(ij)T} - diag(H^{(ij)})\right]$ *with* $H^{(ij)} = \Sigma_{\mathbf{z}_i\mathbf{z}_i}^{-1}\mathbf{e}_{q_i+1}\Sigma_{x_j\mathbf{z}_i}\Sigma_{\mathbf{z}_i\mathbf{z}_i}^{-1}$,

*(ii)* $\left(\frac{\partial\theta_{ij}}{\partial\Sigma_{x_j\mathbf{z}_i}}\right)^T = \frac{\partial\theta_{ij}}{\partial\Sigma_{\mathbf{z}_i x_j}} = \Sigma_{\mathbf{z}_i\mathbf{z}_i}^{-1}\mathbf{e}_{q_i+1}$*, and*

*(iii) All other entries of* $\frac{\partial\theta_{ij}}{\partial\Sigma}$ *are zero.*

PROOF. By the definition via regression coefficients, $\theta_{ij} = \mathbf{e}_{q_i+1}^T\Sigma_{\mathbf{z}_i\mathbf{z}_i}^{-1}\Sigma_{\mathbf{z}_i x_j}$, since $X_j \notin \mathbf{PA}_i$, for $i \in \{1,2\}$, $j \in \{1,2,p\}$ and $i \neq j$. Therefore, (i) follows

from the following matrix calculus result (e.g., [5]): Suppose that $S$ is a symmetric matrix of variables and $\mathbf{a}$ and $\mathbf{b}$ are column vectors, whose entries do not depend on $S$, then

$$\frac{\partial \mathbf{a}^T S^{-1}\mathbf{b}}{\partial S} = -[S^{-1}\mathbf{a}\mathbf{b}^T S^{-1} + (S^{-1}\mathbf{a}\mathbf{b}^T S^{-1})^T - diag(S^{-1}\mathbf{a}\mathbf{b}^T S^{-1})].$$

Part (ii) follows from straightforward differentiation and (iii) follows from the fact that $\theta_{ij}$ is a function of only the entries of $\Sigma_{\mathbf{z}_i\mathbf{z}_i}$ and $\Sigma_{\mathbf{z}_i x_j}$. □

**Proof of Theorem 4.2 of the main text.** Proposition 8.2 shows that $\Sigma^{[1]}$ can be expressed in terms of $\Sigma$. Therefore, equation (8) of the main text and the multivariate delta-method imply

$$\sqrt{n}(\text{vech}(\hat{\Sigma}^{[1]}) - \text{vech}(\Sigma^{[1]})) \xrightarrow{d} \mathcal{N}\left(\mathbf{0}, \Lambda^{[1]}\Gamma\Lambda^{[1]T}\right),$$

where $\Lambda^{[1]} = \frac{\partial \text{vech}(\Sigma^{[1]})}{\partial \text{vech}(\Sigma)}$.

Since $\text{vech}(P\Sigma^{[1]}P^T) = \Pi \ \text{vech}(\Sigma^{[1]})$ and $\text{vech}(P\hat{\Sigma}^{[1]}P^T) = \Pi \ \text{vech}(\hat{\Sigma}^{[1]})$,

$$\sqrt{n}(\text{vech}(P\hat{\Sigma}^{[1]}P^T) - \text{vech}(P\Sigma^{[1]}P^T)) \xrightarrow{d} \mathcal{N}\left(\mathbf{0}, \Pi\Lambda^{[1]}\Gamma\Lambda^{[1]T}\Pi^T\right).$$

Finally, $\Sigma^{[2]}$ can be expressed in terms of $P\Sigma^{[1]}P^T$, so that the final result follows from one more application of the multivariate delta-method. □

Our next goal is to derive a more explicit expression for $\Lambda^{[1]} = \frac{\partial \text{vech}(\Sigma^{[1]})}{\partial \text{vech}(\Sigma)}$. An expression for $\Lambda^{[2]}$ can be derived analogously, and together these expressions can be used to compute the asymptotic variance of the MCD estimator for a given simulation setting. These results will be used in Section 9.

We first write $\Sigma^{[1]}$ as an explicit function of $\Sigma$ in Proposition 8.2. (We will also use this proposition to establish high-dimensional consistency of the MCD estimator when the parent sets are unknown, see Section 6 of the main text)

Proposition 8.2. *(Expressing $\Sigma^{[1]}$ as a function of $\Sigma$) Let $\mathbf{Z}_1 = \mathbf{PA}_1 \cup \{X_1\}$ and $\mathbf{W}_1 = \mathbf{U} \setminus \mathbf{Z}_1$. Assume that the variables in $\Sigma$ and $\Sigma^{[1]}$ are ordered as $(\mathbf{PA}_1, X_1, \mathbf{W}_1)$, where the ordering within $\mathbf{PA}_1$ and $\mathbf{W}_1$ is arbitrary. Then*

$$\Sigma^{[1]} = \begin{pmatrix} \Sigma^{[1]}_{\mathbf{z}_1\mathbf{z}_1} & \Sigma^{[1]}_{\mathbf{z}_1\mathbf{z}_1}\Sigma^{-1}_{\mathbf{z}_1\mathbf{z}_1}\Sigma_{\mathbf{z}_1\mathbf{w}_1} \\ \Sigma_{\mathbf{w}_1\mathbf{z}_1}\Sigma^{-1}_{\mathbf{z}_1\mathbf{z}_1}\Sigma^{[1]}_{\mathbf{z}_1\mathbf{z}_1} & \begin{matrix}\Sigma_{\mathbf{w}_1\mathbf{w}_1} - \Sigma_{\mathbf{w}_1\mathbf{z}_1}\Sigma^{-1}_{\mathbf{z}_1\mathbf{z}_1}\Sigma_{\mathbf{z}_1\mathbf{w}_1} \\ +\Sigma_{\mathbf{w}_1\mathbf{z}_1}\Sigma^{-1}_{\mathbf{z}_1\mathbf{z}_1}\Sigma^{[1]}_{\mathbf{z}_1\mathbf{z}_1}\Sigma^{-1}_{\mathbf{z}_1\mathbf{z}_1}\Sigma_{\mathbf{z}_1\mathbf{w}_1}\end{matrix} \end{pmatrix}, \tag{2}$$

*where*

$$\Sigma^{[1]}_{\mathbf{z}_1\mathbf{z}_1} = \begin{pmatrix} \Sigma_{\mathbf{pa}_1\mathbf{pa}_1} & 0 \\ 0 & \Sigma_{x_1x_1} - \Sigma_{x_1\mathbf{pa}_1}\Sigma^{-1}_{\mathbf{pa}_1\mathbf{pa}_1}\Sigma_{\mathbf{pa}_1x_1} \end{pmatrix}. \tag{3}$$

*Moreover, we can write* $\Sigma^{[1]} = Q^{[1]}\Sigma$*, where* $Q^{[1]}$ *is the following* $q \times q$ *matrix:*

$$Q^{[1]} = \begin{pmatrix} H^{[1]} & \mathbf{0} \\ \Sigma_{\mathbf{w}_1\mathbf{z}_1}\Sigma^{-1}_{\mathbf{z}_1\mathbf{z}_1}(H^{[1]} - \mathrm{I}) & \mathrm{I} \end{pmatrix} \quad \textit{and } H^{[1]} = \Sigma^{[1]}_{\mathbf{z}_1\mathbf{z}_1}\Sigma^{-1}_{\mathbf{z}_1\mathbf{z}_1}.$$

PROOF. Let $L\Sigma L^T = D$ be the Cholesky decomposition of $\Sigma$ and let $\tilde{L}$ be the modification of $L$ produced by Algorithm 3.1 of the main text. Then, by definition, $\Sigma^{[1]} = \tilde{L}^{-1}D\tilde{L}^{-T}$. It can be checked easily that

$$\tilde{L}^{-1} = \begin{pmatrix} \tilde{L}^{-1}_{\mathbf{z}_1\mathbf{z}_1} & 0 \\ -\tilde{L}^{-1}_{\mathbf{w}_1\mathbf{w}_1}\tilde{L}_{\mathbf{w}_1\mathbf{z}_1}\tilde{L}^{-1}_{\mathbf{z}_1\mathbf{z}_1} & \tilde{L}^{-1}_{\mathbf{w}_1\mathbf{w}_1} \end{pmatrix} = \begin{pmatrix} \tilde{L}^{-1}_{\mathbf{z}_1\mathbf{z}_1} & 0 \\ -L^{-1}_{\mathbf{w}_1\mathbf{w}_1}L_{\mathbf{w}_1\mathbf{z}_1}\tilde{L}^{-1}_{\mathbf{z}_1\mathbf{z}_1} & L^{-1}_{\mathbf{w}_1\mathbf{w}_1} \end{pmatrix},$$

where the last equality follows from $\tilde{L}_{\mathbf{w}_1\mathbf{z}_1} = L_{\mathbf{w}_1\mathbf{z}_1}$ and $\tilde{L}_{\mathbf{w}_1\mathbf{w}_1} = L_{\mathbf{w}_1\mathbf{w}_1}$. Hence,

$$\begin{aligned}
\Sigma^{[1]}_{\mathbf{z}_1\mathbf{z}_1} &= \tilde{L}^{-1}_{\mathbf{z}_1\mathbf{z}_1}D_{\mathbf{z}_1\mathbf{z}_1}\tilde{L}^{-T}_{\mathbf{z}_1\mathbf{z}_1}, \\
\Sigma^{[1]}_{\mathbf{w}_1\mathbf{z}_1} &= -L^{-1}_{\mathbf{w}_1\mathbf{w}_1}L_{\mathbf{w}_1\mathbf{z}_1}\tilde{L}^{-1}_{\mathbf{z}_1\mathbf{z}_1}D_{\mathbf{z}_1\mathbf{z}_1}\tilde{L}^{-T}_{\mathbf{z}_1\mathbf{z}_1} = -L^{-1}_{\mathbf{w}_1\mathbf{w}_1}L_{\mathbf{w}_1\mathbf{z}_1}\Sigma^{[1]}_{\mathbf{z}_1\mathbf{z}_1} \quad \text{and} \\
\Sigma^{[1]}_{\mathbf{w}_1\mathbf{w}_1} &= L^{-1}_{\mathbf{w}_1\mathbf{w}_1}L_{\mathbf{w}_1\mathbf{z}_1}\tilde{L}^{-1}_{\mathbf{z}_1\mathbf{z}_1}D_{\mathbf{z}_1\mathbf{z}_1}\tilde{L}^{-T}_{\mathbf{z}_1\mathbf{z}_1}L^T_{\mathbf{w}_1\mathbf{z}_1}L^{-T}_{\mathbf{w}_1\mathbf{w}_1} + L^{-1}_{\mathbf{w}_1\mathbf{w}_1}D_{\mathbf{w}_1\mathbf{w}_1}L^{-T}_{\mathbf{w}_1\mathbf{w}_1} \\
&= L^{-1}_{\mathbf{w}_1\mathbf{w}_1}L_{\mathbf{w}_1\mathbf{z}_1}\Sigma^{[1]}_{\mathbf{z}_1\mathbf{z}_1}L^T_{\mathbf{w}_1\mathbf{z}_1}L^{-T}_{\mathbf{w}_1\mathbf{w}_1} + L^{-1}_{\mathbf{w}_1\mathbf{w}_1}D_{\mathbf{w}_1\mathbf{w}_1}L^{-T}_{\mathbf{w}_1\mathbf{w}_1}.
\end{aligned}$$

Therefore, (2) follows from the following identities that can be derived similarly by considering the Cholesky decomposition $\Sigma = L^{-1}DL^{-T}$:

(i) $\Sigma_{\mathbf{w}_1\mathbf{z}_1} = -L^{-1}_{\mathbf{w}_1\mathbf{w}_1}L_{\mathbf{w}_1\mathbf{z}_1}\Sigma_{\mathbf{z}_1\mathbf{z}_1}$ and
(ii) $\Sigma_{\mathbf{w}_1\mathbf{w}_1} = \Sigma_{\mathbf{w}_1\mathbf{z}_1}\Sigma^{-1}_{\mathbf{z}_1\mathbf{z}_1}\Sigma_{\mathbf{z}_1\mathbf{z}_1}\Sigma^{-1}_{\mathbf{z}_1\mathbf{z}_1}\Sigma^{-1}_{\mathbf{z}_1\mathbf{w}_1} + L^{-1}_{\mathbf{w}_1\mathbf{w}_1}D_{\mathbf{w}_1\mathbf{w}_1}L^{-T}_{\mathbf{w}_1\mathbf{w}_1}$.

To prove (3), we write

$$L_{\mathbf{z}_1\mathbf{z}_1} = \begin{pmatrix} L_{\mathbf{pa}_1\mathbf{pa}_1} & \mathbf{0} \\ L_{x_1\mathbf{pa}_1} & 1 \end{pmatrix}.$$

Similar computations as before lead to $\Sigma_{\mathbf{pa}_1\mathbf{pa}_1} = L^{-1}_{\mathbf{pa}_1\mathbf{pa}_1}D_{\mathbf{pa}_1\mathbf{pa}_1}L^{-T}_{\mathbf{pa}_1\mathbf{pa}_1}$ and $\Sigma_{x_1x_1} = \Sigma_{x_1\mathbf{pa}_1}\Sigma^{-1}_{\mathbf{pa}_1\mathbf{pa}_1}\Sigma_{\mathbf{pa}_1x_1} + D_{x_1x_1}$. This completes the proof of (3), since

$$\begin{aligned}
\Sigma^{[1]}_{\mathbf{z}_1\mathbf{z}_1} &= \begin{pmatrix} L^{-1}_{\mathbf{pa}_1\mathbf{pa}_1} & \mathbf{0} \\ \mathbf{0}^T & 1 \end{pmatrix}\begin{pmatrix} D_{\mathbf{pa}_1\mathbf{pa}_1} & \mathbf{0} \\ \mathbf{0}^T & D_{x_1x_1} \end{pmatrix}\begin{pmatrix} L^{-T}_{\mathbf{pa}_1\mathbf{pa}_1} & \mathbf{0} \\ \mathbf{0}^T & 1 \end{pmatrix} \\
&= \begin{pmatrix} L^{-1}_{\mathbf{pa}_1\mathbf{pa}_1}D_{\mathbf{pa}_1\mathbf{pa}_1}L^{-T}_{\mathbf{pa}_1\mathbf{pa}_1} & \mathbf{0} \\ \mathbf{0}^T & D_{x_1x_1} \end{pmatrix}.
\end{aligned}$$

Finally, one can check that $Q^{[1]}\Sigma$ equals the right hand side of (2). □

We now continue our derivation of $\Lambda^{[1]}$. Note that $\mathbf{PA}_1 = \emptyset$ implies $\Sigma^{[1]} = \Sigma$ and $\Lambda^{[1]}$ is the identity matrix in this case. Hence, we assume $|\mathbf{PA}_1| = q_1 \geq 1$.

Note that the $j$-th column of $\Lambda^{[1]}$ can be written as

$$\Lambda^{[1]}_{*j} = \frac{\partial \mathrm{vech}(\Sigma^{[1]})}{\partial \Sigma_{rs}} = \mathrm{vech}\left(\frac{\partial \Sigma^{[1]}}{\partial \Sigma_{rs}}\right),$$

where $1 \leq s \leq r \leq q$ are unique numbers such that for any $q \times q$ symmetric matrix $A$, $A_{rs} = \mathrm{vech}(A)_j$. We therefore only derive an expression for the derivative of $\Sigma^{[1]}$ with respect to $\Sigma_{rs}$:

$$\frac{\partial \Sigma^{[1]}}{\partial \Sigma_{rs}} = \frac{\partial Q^{[1]}}{\partial \Sigma_{rs}} \Sigma + Q^{[1]} E^{rs},$$

where we define $E^{rs}$ to be a symmetric matrix of appropriate dimensions with $E^{rs}_{ij} = 0$, if $(i,j) \notin \{(r,s),(s,r)\}$ and $E^{rs}_{rs} = E^{rs}_{sr} = 1$.

Next, we derive an expression for $\frac{\partial Q^{[1]}}{\partial \Sigma_{rs}}$. The definition of $Q^{[1]}$ implies

$$\frac{\partial Q^{[1]}}{\partial \Sigma_{rs}} = \begin{pmatrix} \frac{\partial H^{[1]}}{\partial \Sigma_{rs}} & \mathbf{0} \\ \frac{\partial \Sigma_{\mathbf{w}_1\mathbf{z}_1}\Sigma^{-1}_{\mathbf{z}_1\mathbf{z}_1}}{\partial \Sigma_{rs}} (H^{[1]} - \mathrm{I}) + \Sigma_{\mathbf{w}_1\mathbf{z}_1}\Sigma^{-1}_{\mathbf{z}_1\mathbf{z}_1} \frac{\partial H^{[1]}}{\partial \Sigma_{rs}} & \mathbf{0} \end{pmatrix}.$$

For any symmetric matrix $A$, we have $\frac{\partial A^{-1}}{\partial A_{rs}} = -A^{-1}E^{rs}A^{-1}$. Hence,

$$\frac{\partial \Sigma_{\mathbf{w}_1\mathbf{z}_1}\Sigma^{-1}_{\mathbf{z}_1\mathbf{z}_1}}{\partial \Sigma_{rs}} = \begin{cases} -\Sigma_{\mathbf{w}_1\mathbf{z}_1}\Sigma^{-1}_{\mathbf{z}_1\mathbf{z}_1} E^{rs} \Sigma^{-1}_{\mathbf{z}_1\mathbf{z}_1} & \text{if } s, r \leq q_1 + 1, \\ E^{rs}_{\mathbf{w}_1\mathbf{z}_1}\Sigma^{-1}_{\mathbf{z}_1\mathbf{z}_1} & \text{if } s \leq q_1 + 1 < r, \\ \mathbf{0} & \text{otherwise.} \end{cases}$$

Finally,

$$\frac{\partial H^{[1]}}{\partial \Sigma_{rs}} = \begin{cases} \frac{\partial \Sigma^{[1]}_{\mathbf{z}_1\mathbf{z}_1}}{\partial \Sigma_{rs}} \Sigma^{-1}_{\mathbf{z}_1\mathbf{z}_1} - \Sigma^{[1]}_{\mathbf{z}_1\mathbf{z}_1}\Sigma^{-1}_{\mathbf{z}_1\mathbf{z}_1} E^{rs} \Sigma^{-1}_{\mathbf{z}_1\mathbf{z}_1} & \text{if } s, r \leq q_1 + 1, \\ \mathbf{0} & \text{otherwise,} \end{cases}$$

where, for $s, r \leq q_1 + 1$,

$$\frac{\partial \Sigma^{[1]}_{\mathbf{z}_1\mathbf{z}_1}}{\partial \Sigma_{rs}} = \begin{pmatrix} E^{rs} 1_{\{r,s \leq q_1\}} & \mathbf{0} \\ \mathbf{0}^T & \frac{\partial \Sigma^{[1]}_{x_1 x_1}}{\partial \Sigma_{rs}} \end{pmatrix}$$

with

$$\frac{\partial \Sigma^{[1]}_{x_1 x_1}}{\partial \Sigma_{rs}} = \begin{cases} \Sigma_{x_1\mathbf{pa}_1}\Sigma^{-1}_{\mathbf{pa}_1\mathbf{pa}_1} E^{rs} \Sigma^{-1}_{\mathbf{pa}_1\mathbf{pa}_1}\Sigma_{\mathbf{pa}_1 x_1} & \text{if } r, s \leq q_1, \\ -2\mathbf{e}^T_{\min(r,s)}\Sigma^{-1}_{\mathbf{pa}_1\mathbf{pa}_1}\Sigma_{\mathbf{pa}_1 x_1} & \text{if } s \leq q_1,\ r = q_1 + 1\ , \\ 1 & \text{if } r = s = q_1 + 1. \end{cases}$$

**9. Numerical comparison of asymptotic variances.** We use the R-package **pcalg** [9] to simulate $n_{iter}$ random weighted DAGs with $p$ vertices, a pre-specified expected neighborhood size $ens$, and edge weights that are drawn independently from a Uniform$[0, ul]$ distribution. We choose the error variables to be normally distributed, where the variances are drawn independently from a Uniform$[1, 2]$ distribution. For each $t = 1, \ldots, n_{iter}$, the weighted DAG $\mathcal{G}^{(t)}$ with weight matrix $B^{(t)}$ and the vector of error variables $\boldsymbol{\epsilon}^{(t)}$ define a distribution on $\mathbf{X}^{(t)} = (X_1^{(t)}, \ldots, X_p^{(t)})^T$ that satisfies $\mathbf{X}^{(t)} = (B^{(t)})^T \mathbf{X}^{(t)} + \boldsymbol{\epsilon}^{(t)}$. For each $t = 1, \ldots, n_{iter}$, we randomly choose a pair of intervention nodes $\{X_{i_t}^{(t)}, X_{j_t}^{(t)}\}$ and a response variable $X_{r_t}^{(t)}$ such that $X_{r_t}^{(t)} \notin \mathbf{PA}_{i_t}(\mathcal{G}^{(t)}) \cup \mathbf{PA}_{j_t}(\mathcal{G}^{(t)})$.

We compare the asymptotic variances of RRC and MCD in three simulation settings:

**Setting 1:** $p = 10,\ ens = 1.5,\ ul = 1$;
**Setting 2:** $p = 10,\ ens = 3,\ ul = 1$;
**Setting 3:** $p = 10,\ ens = 1.5,\ ul = 1.5$.

For each setting, we perform $n_{iter} = 500$ iterations and compute the asymptotic variances of the RRC estimators $\hat{\theta}_{i_t r_t}^{(i_t, j_t)}(\mathcal{G}^{(t)})$ and $\hat{\theta}_{j_t r_t}^{(i_t, j_t)}(\mathcal{G}^{(t)})$ and the MCD estimators $\tilde{\theta}_{i_t r_t}^{(i_t, j_t)}(\mathcal{G}^{(t)})$ and $\tilde{\theta}_{j_t r_t}^{(i_t, j_t)}(\mathcal{G}^{(t)})$, for each $t = 1, \ldots, n_{iter}$, using the formulas in Theorem 4.1 and Corollary 4.1 of the main text.

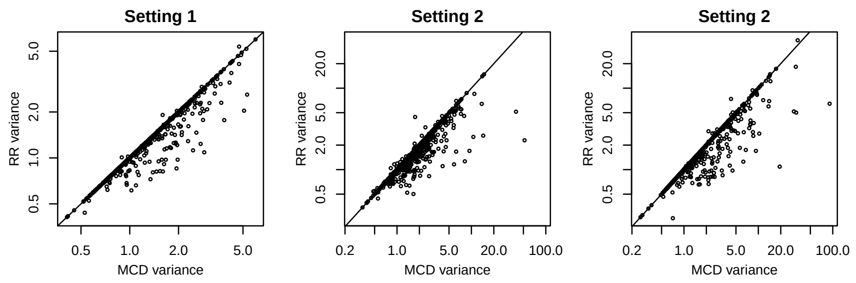


Fig 6: Log-log plots of asymptotic variances of the RRC and MCD estimators for the chosen triples $(X_{i_t}^{(t)}, X_{j_t}^{(t)}, X_{r_t}^{(t)})$, $t = 1, \ldots, n_{iter}$. (See also Section 4 of the main text.)

The plots in Figure 6 show that no estimator dominates the other asymptotically but RRC seems to have a smaller asymptotic variance in most cases. Note that the scale in the leftmost plot is different from the other two plots. The leftmost plot indicates that if the underlying DAG is sparse and the edge weights are small, RRC and MCD are asymptotically similar

with a slight advantage for RRC. On the other hand, the second and third plots show that the asymptotic similarity decreases as the underlying DAG becomes more dense or the edge weights become larger.

## 10. Proof of Theorem 5.1 of the main text.

**Proof of Theorem 5.1 of the main text.** Let $\mathcal{C}_1, \dots, \mathcal{C}_r$ denote the connected components of $\mathcal{C}_{undir}$, where they are ordered such that each of $\mathcal{C}_1, \dots, \mathcal{C}_s$ contains at least one intervention node, and $\mathcal{C}_{s+1}, \dots, \mathcal{C}_r$ contain no intervention nodes ($1 \leq s \leq r$). Recall that no orientation of edges not oriented in $\mathcal{C}$ can create a directed cycle or a new v-structure that includes at least one edge that was oriented in $\mathcal{C}$ (see the proof of Theorem 4 in [13]). Therefore, each $\mathcal{C}_i$, $i = 1, \dots, r$, must be a CPDAG and can be oriented independently of the other undirected connected components. Let $m_i$ denote the number of DAGs in the Markov equivalence class represented by $\mathcal{C}_i$. Now since each element of the multiset $\mathcal{PA}_{s\ell}$ corresponds to an orientation of edges in $\mathcal{C}_1, \dots, \mathcal{C}_s$, each element of the multiset $\mathcal{PA}_{s\ell}$ is repeated $\prod_{i=s+1}^{r} m_i$ times (which is the total number of valid orientations of $\mathcal{C}_{s+1}, \dots, \mathcal{C}_r$) in the multiset $\mathcal{PA}_{all}$. □

**11. Numerical comparison of computation times.** We compare computation times of the semi-local algorithm (Algorithm 5.1 of the main text) for single interventions and the local algorithm of IDA. To this end, we randomly generate 100 DAGs as in Section 9, with $p = 1000$ and $ens = 4$. For each CPDAG that represents the Markov equivalence class of a generated DAG, we randomly choose 100 nodes for obtaining their parent sets separately using the semi-local algorithm and the local algorithm of IDA, each time recording the computation time. Figure 7 shows that the computation time of the semi-local algorithm (excluding outliers) is comparable to that of the local algorithm of IDA. However, in a few cases, which are not shown in the boxplot, the semi-local algorithm took extremely long to determine all parent sets of an intervention node. We encountered 1.05% cases where the semi-local algorithm took more than 1 second, with a median equal to 15 seconds. Those are the cases where the intervention node belongs to a moderately large connected component (e.g., containing more than 8 nodes) of the undirected subgraph of the corresponding CPDAG. We used the `allDags()` function of the R-package **pcalg** [9] to obtain all DAGs in the Markov equivalence class of an undirected connected component. Note that obtaining all DAGs in a Markov equivalence class takes exponential time and thus quickly becomes infeasible. We did not record computation time when a connected component had more than 12 nodes, a

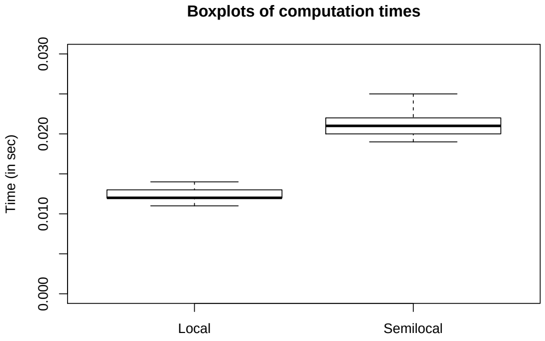


Fig 7: Boxplots of computation times (in seconds) of the local algorithm and the semi-local algorithm for single interventions (outliers excluded). (See also Section 5 of the main text.)

situation that occurred only in 0.12% cases.

**12. Sample version of Algorithm 5.1 of the main text.** There are various existing methods to estimate CPDAGs. Score-based methods, such as GES [2], aim to obtain a CPDAG that optimizes a score function (e.g., BIC). On the other hand, constraint-based method, such as the PC-algorithms [20], are based on conditional independence tests. Recently, an order independent version of the PC algorithm has been proposed [4] and it has been empirically shown to improve estimation quality. Rank-PC [6] is another variant of the PC algorithm which is based on rank correlations. Rank-PC is empirically shown to be more robust than PC under non-Gaussian errors [6]. The PC-algorithm and its variants scale well with the number of variables and they have been shown to be consistent in certain sparse high-dimensional settings [4, 6, 8]. We therefore recommend using an order independent modification of the PC algorithm or the Rank-PC algorithm.

The output of the sample version of the PC-algorithm (or its variants) is not necessarily a PDAG, since it can contain directed cycles due to testing errors. Moreover, even if the output is a PDAG, it does not need to be a CPDAG in the sense that it represents a Markov equivalence class of DAGs. In particular, if one of the undirected components of the estimated CPDAG $\hat{\mathcal{C}}$ is non-chordal, then it is impossible to orient the undirected edges without creating additional directed cycles or additional v-structures.

In all these cases, we cannot determine jointly valid parent sets. Algorithm

5.1 of the main text, however, can still be used if and only if $\hat{\mathcal{C}}_1, \ldots, \hat{\mathcal{C}}_s$ are all chordal. We therefore propose the following modification in the sample version of Algorithm 5.1 of the main text. We simply run the algorithm with the estimated CPDAG as input, with the following difference in step 3: if $\hat{\mathcal{C}}_i$ is non-chordal, then we obtain $\mathcal{PA}_i$ by combining all locally valid parent sets of the intervention nodes in $\hat{\mathcal{C}}_i$ (as in Example 3 of the main text). (There are of course other possible solutions. For example, one could also add edges to any non-chordal component $\hat{\mathcal{C}}_i$ to make it chordal or one can perform a score based search in a local neighborhood of the estimated graph to obtain an optimal CPDAG.)

## 13. An example for estimating the multiset of causal effects when the CPDAG is known.

Example 6. *We consider the DAG $\mathcal{G}$ given in Example 1 of the main text, and generate $n_{iter} = 1000$ samples of size $n_{samp} = 1000$, letting $\epsilon_1, \ldots, \epsilon_6$ be i.i.d. standard Normal random variables.*

*We want to estimate the multi-set of possible total effects of $X_i$ $(i = 1, 2)$ on $X_6$ in a joint intervention on $(X_1, X_2)$, defined as*

$$\Theta_{i6}^{(1,2)} := \{\theta_{i6}^{(1,2)}(\mathbf{PA}') : \mathbf{PA}' \in \mathcal{PA}_{s\ell}\}.$$

*We first determine the true values $\Theta_{16}^{(1,2)}$ and $\Theta_{26}^{(1,2)}$. To this end, note that the CPDAG $\mathcal{C}$ that represents $\mathcal{G}$ is as $\mathcal{G}$ but with undirected edges $5 - 1$ and $1 - 3$. Hence, using Algorithm 5.1 of the main text, the possible jointly valid parent sets of $(1, 2)$ are*

$$\mathcal{PA}_{s\ell} = \{(\{5\}, \{3, 4\}), (\emptyset, \{3, 4\}), (\{3\}, \{3, 4\})\}.$$

*Note that for all $\mathbf{PA}' \in \mathcal{PA}_{s\ell}$, $\theta_{26}^{(1,2)}(\mathbf{PA}') = 0.4$, while $\theta_{16}^{(1,2)}(\mathbf{PA}') = 0$ for $\mathbf{PA}' = (\{3\}, \{3, 4\})$ and $\theta_{16}^{(1,2)}(\mathbf{PA}') = 0.99$ otherwise. Hence,*

$$\Theta_{16}^{(1,2)} = \{0.99, 0.99, 0\} \quad \text{and} \quad \Theta_{26}^{(1,2)} = \{0.4, 0.4, 0.4\}.$$

*For each $t = 1, \ldots, n_{iter}$, we compute estimates of $\Theta_{16}^{(1,2)}$ and $\Theta_{26}^{(1,2)}$ under the assumption that the true CPDAG is known, by applying RRC, MCD and IPW for each $\mathbf{PA}' \in \mathcal{PA}_{s\ell}$ (the output of Algorithm 5.1 of the main text). We construct density plots of the estimates of the multiset $\Theta_{i6}^{(1,2)}$, where we combine all $3 \times n_{iter}$ estimates to estimate the density for each of the three methods, for $i = 1, 2$. The plots in Figure 8 show that RRC and MCD outperform IPW, both in terms of bias and variance. RRC and MCD seem to have similar performance.*

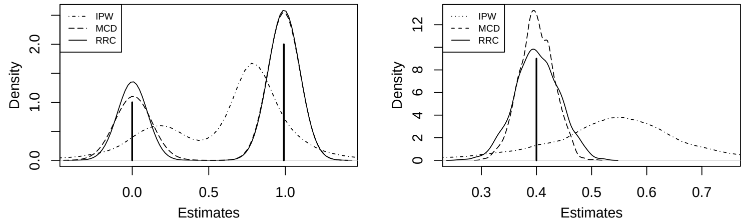


Fig 8: Density plots of estimates of $\Theta_{16}^{(1,2)}$ (left panel) and $\Theta_{26}^{(1,2)}$ (right panel) based on IPW, MCD and RRC. The vertical bars indicate true values and the heights of the bars are proportional to the corresponding multiplicities. (See also Section 6 of the main text.)

**14. Low-dimensional simulation with Gaussian errors.** We randomly generate $n_{iter} = 5000$ weighted DAGs as in Section 9, with $p = 6$ vertices and expected neighborhood size $ens = 3$. The edge weights are drawn independently from a Uniform$[0.2, 1.2]$ distribution. The error variables are distributed as standard normal random variables. For each $t = 1, \dots, n_{iter}$, we generate standardized data by using the true correlation matrix $R^{(t)}$ of $\mathbf{X}^{(t)} = (X_1^{(t)}, \dots, X_6^{(t)})^T$ as the covariance matrix to generate $n_{samp} = 1000$ i.i.d. observations from $\mathcal{N}(0, R^{(t)})$.

For each $t = 1, \dots, n_{iter}$, we randomly choose a pair of intervention nodes $\{X_{i_t}^{(t)}, X_{j_t}^{(t)}\}$ and a response variable $X_{r_t}^{(t)}$ such that $X_{r_t}^{(t)} \notin \mathbf{PA}_{i_t}(\mathcal{G}^{(t)}) \cup \mathbf{PA}_{j_t}(\mathcal{G}^{(t)})$. Then we compute the multisets of total joint effects $\Theta_{i_t r_t}^{(i_t,j_t)}(\mathcal{C}^{(t)})$ and $\Theta_{j_t r_t}^{(i_t,j_t)}(\mathcal{C}^{(t)})$, using the CPDAG $\mathcal{C}^{(t)}$ that corresponds to $\mathcal{G}^{(t)}$ and the covariance matrix $R^{(t)}$. We aim to estimate two summary measures of these sets: the minimum absolute value (minabs) and the average (aver).

We consider two scenarios: (i) the true CPDAG is known and we use the data only in step 3 of Algorithm 6.1 of the main text, and (ii) the CPDAG is estimated from the data, using the order independent version of the PC-algorithm [4] with tuning parameter $\alpha = 0.01$.

For $t = 1, \dots, n_{iter}$ and $\ell = i_t, j_t$, we compute the errors for estimating minabs$(\Theta_{\ell r_t}^{(i_t,j_t)}(\mathcal{C}^{(t)}))$ and aver$(\Theta_{\ell r_t}^{(i_t,j_t)}(\mathcal{C}^{(t)}))$ using the joint-IDA estimators based on RRC, MCD and IPW [18].

For minabs$(\Theta_{\ell r_t}^{(i_t,j_t)}(\mathcal{C}^{(t)})) < 0.1$ and $|$aver$(\Theta_{\ell r_t}^{(i_t,j_t)}(\mathcal{C}^{(t)}))| < 0.1$, the densities of the estimation errors are shown in Figure 9a. We see that RRC and MCD perform about equally well and outperform IPW for both summary measures. However, the performances of the three methods are roughly equal when the CPDAG is estimated. This can be explained by the fact that the

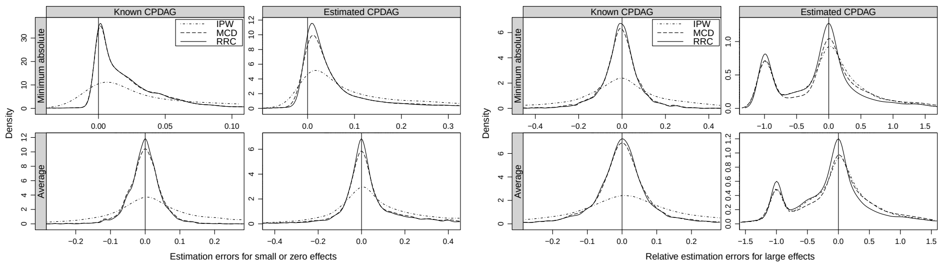


(a) (b)

Fig 9: Density plots of the (relative) errors for estimating $\mathrm{minabs}(\Theta^{(i_t,j_t)}_{\ell r_t}(\mathcal{C}^{(t)}))$ (upper panels) and $\mathrm{aver}(\Theta^{(i_t,j_t)}_{\ell r_t}(\mathcal{C}^{(t)}))$ (lower panels) for $\ell = i_t, j_t$ and $t = 1, \ldots, n_{iter}$, when the CPDAG is known (left panels) and when the CPDAG is estimated (right panels). Subfigure (a) corresponds to the cases where $\mathrm{minabs}(\Theta^{(i_t,j_t)}_{\ell r_t}(\mathcal{C}^{(t)})) < 0.1$ and $|\mathrm{aver}(\Theta^{(i_t,j_t)}_{\ell r_t}(\mathcal{C}^{(t)}))| < 0.1$, while subfigure (b) corresponds $\mathrm{minabs}(\Theta^{(i_t,j_t)}_{\ell r_t}(\mathcal{C}^{(t)})) \geq 0.1$ and $|\mathrm{aver}(\Theta^{(i_t,j_t)}_{\ell r_t}(\mathcal{C}^{(t)}))| \geq 0.1$. (See also Section 6.1 of the main text.)

error coming from the estimation of the CPDAG is significant and common to all three methods.

For $\mathrm{minabs}(\Theta^{(i_t,j_t)}_{\ell r_t}(\mathcal{C}^{(t)})) \geq 0.1$ and $|\mathrm{aver}(\Theta^{(i_t,j_t)}_{\ell r_t}(\mathcal{C}^{(t)}))| \geq 0.1$, the densities of the relative errors are shown in Figure 9b. We see that RRC and MCD perform about equally well and outperform IPW for both summary measures when the CPDAG is known. However, the performances of all three methods are similar when the CPDAG is estimated. Moreover, in this case, relative errors have bimodal densities for both summary measures. The peak at the value $-1$ occurs due to non-zero effects where we assigned zero values whenever a response variable was a parent of an intervention variable in the (wrongly) estimated CPDAG.

**15. Assumptions (A5*) and (A5') of Section 6.2 of the main text.** Assumption (A5*) is stronger than (A5): if (A5*) is satisfied with $v^*$, then (A5) is also satisfied with $v^*$. This is because $\mathrm{Var}(X_{nj}|\mathbf{PA}_i(\mathcal{G}_{nr})) \geq \mathrm{Var}(X_{nj}|X_i, \mathbf{PA}_i(\mathcal{G}_{nr}))$. Assumption (A5*) additionally ensures that $\theta_{ij}(\mathcal{G}_{nr})$ is uniformly bounded for all $n$, where $\theta_{ij}(\mathcal{G}_{nr})$ is the total effect of $X_{ni}$ on

$X_{nj}$ in the DAG $\mathcal{G}_{nr}$. To see this, note that the law of total variance implies

$$\begin{aligned}
&\mathrm{Var}(X_{nj}|\mathbf{PA}_i(\mathcal{G}_{nr})) \\
=&\mathrm{E}[\mathrm{Var}(X_{nj}|X_{ni}, \mathbf{PA}_i(\mathcal{G}_{nr}))|\mathbf{PA}_i(\mathcal{G}_{nr})] + \mathrm{Var}(\mathrm{E}[X_{nj}|X_i, \mathbf{PA}_i(\mathcal{G}_{nr})]|\mathbf{PA}_i(\mathcal{G}_{nr})) \\
=&\mathrm{Var}(X_{nj}|X_{ni}, \mathbf{PA}_i(\mathcal{G}_{nr})) + (\theta_{ij}(\mathcal{G}_{nr}))^2 \mathrm{Var}(X_{ni}|\mathbf{PA}_i(\mathcal{G}_{nr})),
\end{aligned}$$

where the last equality follows from the assumption that the distribution of $\mathbf{X}_n$ is multivariate Gaussian, so that the conditional variance does not depend on the values of the conditioning variables and the conditional expectation is a linear function of the conditioning variables. Therefore,

$$\frac{\mathrm{Var}(X_{nj}|\mathbf{PA}_i(\mathcal{G}_{nr}))}{\mathrm{Var}(X_{ni}|\mathbf{PA}_i(\mathcal{G}_{nr}))} = \frac{\mathrm{Var}(X_{nj}|X_{ni}, \mathbf{PA}_i(\mathcal{G}_{nr}))}{\mathrm{Var}(X_{ni}|\mathbf{PA}_i(\mathcal{G}_{nr}))} + (\theta_{ij}(\mathcal{G}_{nr}))^2.$$

Now we argue that Assumption (A5′) is stronger than assumption (A5*). Since the distribution of $\mathbf{X}_n$ is multivariate Gaussian, $\mathrm{Var}(X_{nj}|\mathbf{PA}_i(\mathcal{G}_{nr}))$ can be written as a Schur complement. From the interlacing property of eigenvalues of a Hermitian matrix $A$ and the eigenvalues of the Schur complement of any principal sub-matrix of $A$ (see, e.g., Corollary 2.3 of [25]), it follows that $\mathrm{Var}(X_{nj}|\mathbf{PA}_i(\mathcal{G}_{nr})) \leq \lambda_{\max}(\Sigma_{nijr})$ and $\mathrm{Var}(X_{ni}|\mathbf{PA}_i(\mathcal{G}_{nr})) \geq \lambda_{\min}(\Sigma'_{nijr})$ for all $i < p_n$ and $j \leq p_n$. Hence, assumption (A5′) with $v'$ implies assumption (A5*) with $v'$. The main reason for imposing (A5′) instead of (A5*) is that the proof of Theorem 6.2 of the main text involves covariance matrices rather than regression coefficients.

We note that (A5′) is slightly weaker than requiring a uniformly bounded condition number $\lambda_{\max}(\Sigma_{nijr})/\lambda_{\min}(\Sigma_{nijr})$. The reason for having this slightly weaker assumption is that (A5′) allows the variance of the response variable $X_{np_n}$ to converge to zero as $n \to \infty$, while a uniformly bounded condition number would not allow that.

**16. Proof of Theorem 6.1 of the main text.** Lemma 16.1 below was used to prove asymptotic consistency of IDA for single interventions in high-dimensional settings. Our approach to proving Theorem 6.1 of the main text is similar, but we use Lemma 16.2, which follows from Lemma 16.1.

LEMMA 16.1. *(Theorem 5.1 of [11]) Assume that (A1), (A3) and (A5) hold. Then for $\delta > 0$ and $n \geq N$,*

$$\begin{aligned}
&\sup_{i<p_n, r\leq m_n} \mathbb{P}(|\hat{\theta}_{ip_n}(\mathcal{G}_{nr}) - \theta_{ip_n}(\mathcal{G}_{nr})| > \delta) \\
\leq\ & \frac{C_1}{\delta} \exp\left(-C_2\delta^2(n - q_n - 1)\right) + 2\exp\left(-C_3(n/2 - q_n - 1)\right),
\end{aligned}$$

*where $\hat{\theta}_{ip_n}(\mathcal{G}_{nr})$ is the adjusted regression estimator (see Section 3.3 of the main text) of the total effect of $X_{ni}$ on $X_{np_n}$ assuming that the $\mathbf{PA}_i(\mathcal{G}_{nr})$ is the true parent set of $X_{ni}$, $N$ is a constant depending on $q_n$ (see assumption (A3)), $C_1, C_2 > 0$ are constants depending on $v$ (see assumption (A5)), and $C_3 > 0$ is an absolute constant.*

LEMMA 16.2. *Assume that (A1), (A3) and (A5*) hold. Then for $0 < \delta \leq 1$ and $n \geq N$,*

$$\sup_{i,j<p_n, i\neq j, r\leq m_n} \mathbb{P}(|\hat{\theta}^{(i,j)}_{ip_n}(\mathcal{G}_{nr}) - \theta^{(i,j)}_{ip_n}(\mathcal{G}_{nr})| > \delta)$$
$$\leq \frac{C_1^*}{\delta} \exp\left(-C_2^* \delta^2 (n - q_n - 1)\right) + 2\exp\left(-C_3(n/2 - q_n - 1)\right),$$

*where $N > 0$ is a constant depending on $q_n$, $C_1^*, C_2^* > 0$ are constants depending on $v^*$ (see assumption (A5*)), and $C_3 > 0$ is an absolute constant.*

PROOF. If $X_{np_n} \in \mathbf{PA}_i(\mathcal{G}_{nr})$, then by definition $\hat{\theta}^{(i,j)}_{ip_n}(\mathcal{G}_{nr}) = \theta^{(i,j)}_{ip_n}(\mathcal{G}_{nr}) = 0$. Otherwise, Theorem 3.1 and Definition 3.1 of the main text imply that we can bound the difference between the total joint effect and the estimated total joint effect in terms of the single intervention effects and the corresponding estimates:

$$|\hat{\theta}^{(i,j)}_{ip_n}(\mathcal{G}_{nr}) - \theta^{(i,j)}_{ip_n}(\mathcal{G}_{nr})|$$
$$\leq |\hat{\theta}_{ip_n}(\mathcal{G}_{nr}) - \theta_{ip_n}(\mathcal{G}_{nr})| + |\hat{\theta}_{ij}(\mathcal{G}_{nr})\hat{\theta}_{jp_n}(\mathcal{G}_{nr}) - \theta_{ij}(\mathcal{G}_{nr})\theta_{jp_n}(\mathcal{G}_{nr})|.$$

The second term on the right hand side can be decomposed by applying the standard inequality $|\hat{A}_n\hat{B}_n - A_nB_n| \leq |\hat{A}_n - A_n||\hat{B}_n - B_n| + |A_n||\hat{A}_n - A_n| + |B_n||\hat{B}_n - B_n|$ with $\hat{A}_n = \hat{\theta}_{ij}(\mathcal{G}_{nr})$, $A_n = \theta_{ij}(\mathcal{G}_{nr})$, $\hat{B}_n = \hat{\theta}_{jp_n}(\mathcal{G}_{nr})$ and $B_n = \theta_{jp_n}(\mathcal{G}_{nr})$. We complete the proof by showing that $\theta_{ij}(\mathcal{G}_{nr})$ and $\theta_{jp_n}(\mathcal{G}_{nr})$ are bounded, so that the result follows from Lemma 16.1.

If $X_{nj} \in \mathbf{PA}_i(\mathcal{G}_{nr})$, then $\theta_{ij}(\mathcal{G}_{nr})$ is zero. Otherwise, $\theta_{ij}(\mathcal{G}_{nr})$ equals the regression coefficient of $X_{ni}$ in the regression $X_{nj} \sim X_{ni} + \mathbf{PA}_i(\mathcal{G}_{nr})$, denoted as $\beta_{ij|\mathbf{PA}_i}(\mathcal{G}_{nr})$. Therefore, $\theta^2_{ij}(\mathcal{G}_{nr})$ and $\theta^2_{jp_n}(\mathcal{G}_{nr})$ are bounded by $v^*$ given in (A5*), since $\beta^2_{ij|\mathbf{PA}_i}(\mathcal{G}_{nr}) \leq \mathrm{Var}(X_{nj}|\mathbf{PA}_i(\mathcal{G}_{nr}))/\mathrm{Var}(X_{ni}|\mathbf{PA}_i(\mathcal{G}_{nr}))$. □

The proof of Theorem 6.1 of the main text now follows analogously to the proof of Theorem 5.1 of [11], using Lemma 16.2 instead of Lemma 16.1. We present it for completeness.

**Proof of Theorem 6.1 of the main text.** Let $\mathcal{C}_n$ be the CPDAG that represent the Markov equivalence class of $\mathcal{G}_n$. By consistency of the PC-algorithm, there is a sequence $\alpha_n$ converging to zero such that $\mathbb{P}(A_n) \to 1$

for $A_n = \{\hat{\mathcal{C}}(\alpha_n) = \mathcal{C}_n\}$, where $\hat{\mathcal{C}}(\alpha_n)$ denote the output of the PC-algorithm. Hence, it is sufficient to show that

$$\mathbb{P}\left(\sup_{i,j<p_n, i\neq j} d(\hat{\Theta}_{p_n}^{(i,j)}(\alpha_n), \Theta_{p_n}^{(i,j)}) > \delta, A_n\right) \longrightarrow 0.$$

On the set $A_n$ we have

$$\hat{\Theta}_{p_n}^{(i,j)}(\alpha_n) = \left\{(\hat{\theta}_{ip_n}^{(i,j)}(\mathbf{PA}'), \hat{\theta}_{jp_n}^{(i,j)}(\mathbf{PA}'))^T : \mathbf{PA}' \in \mathcal{PA}_{n,s\ell}^{(i,j)}\right\}.$$

In particular, $\hat{\Theta}_{p_n}^{(i,j)}(\alpha_n)$ does not depend on $\alpha_n$, and $\hat{\Theta}_{p_n}^{(i,j)}$ and $\Theta_{p_n}^{(i,j)}$ have the same cardinality. Let $\hat{\Theta}_{ip_n}^{(i,j)} := \{\hat{\theta}_{ip_n}^{(i,j)}(\mathbf{PA}') : \mathbf{PA}' \in \mathcal{PA}_{n,s\ell}^{(i,j)}\}$ and let $\hat{\Theta}_{jp_n}^{(i,j)}$, $\Theta_{ip_n}^{(i,j)}$ and $\Theta_{jp_n}^{(i,j)}$ be defined similarly. Since pairing of the elements of $\hat{\Theta}_{ip_n}^{(i,j)}$ and $\Theta_{ip_n}^{(i,j)}$ with respect to their order statistics is an optimal pairing for the supremum distance, we have

$$d(\hat{\Theta}_{ip_n}^{(i,j)}, \Theta_{ip_n}^{(i,j)}) \leq \sup_{\mathbf{PA}' \in \mathcal{PA}_{n,s\ell}^{(i,j)}} |\hat{\theta}_{ip_n}^{(i,j)}(\mathbf{PA}') - \theta_{ip_n}^{(i,j)}(\mathbf{PA}')|.$$

The number of distinct elements in $\mathcal{PA}_{n,s\ell}^{(i,j)}$ is bounded above by $2^{|\mathbf{ADJ}_i(\mathcal{G}_n)|} \times 2^{|\mathbf{ADJ}_j(\mathcal{G}_n)|}$ which is bounded by $4^{q_n}$ (see assumption (A3)). Hence,

$$\begin{aligned}
&\mathbb{P}(\sup_{i,j<p_n, i\neq j} d(\hat{\Theta}_{p_n}^{(i,j)}, \Theta_{p_n}^{(i,j)}) > \delta, A_n) \\
\leq& p_n^2 \sup_{i,j<p_n, i\neq j} \mathbb{P}(\sup_{\mathbf{PA}' \in \mathcal{PA}_{n,s\ell}^{(i,j)}} |\hat{\theta}_{ip_n}^{(i,j)}(\mathbf{PA}') - \theta_{ip_n}^{(i,j)}(\mathbf{PA}')| > \delta) \\
\leq& p_n^2\, 4^{q_n} \sup_{\substack{i,j<p_n, i\neq j, \\ \mathbf{PA}' \in \mathcal{PA}_{n,s\ell}^{(i,j)}}} \mathbb{P}(|\hat{\theta}_{ip_n}^{(i,j)}(\mathbf{PA}') - \theta_{ip_n}^{(i,j)}(\mathbf{PA}')| > \delta) \\
=& p_n^2\, 4^{q_n} \sup_{i,j<p_n, i\neq j, r\leq m_n} \mathbb{P}(|\hat{\theta}_{ip_n}^{(i,j)}(\mathcal{G}_{nr}) - \theta_{ip_n}^{(i,j)}(\mathcal{G}_{nr})| > \delta),
\end{aligned}$$

where $\{\mathcal{G}_{n1}, \ldots, \mathcal{G}_{nm_n}\}$ is the Markov equivalence class of $\mathcal{C}_n$, and the last equality follows from the fact that $\mathcal{PA}_{n,s\ell}^{(i,j)} \overset{set}{=} \{\mathbf{PA}_{\{i,j\}}(\mathcal{G}_{nr}) : r \leq m_n\}$. This completes the proof since Lemma 16.2 and assumptions (A2) and (A3) ensure that the last expression converges to zero as $n \to \infty$. □

## 17. Proof of Theorem 6.2 of the main text.

**Proof of Theorem 6.2 of the main text.** In Lemma 17.1 we will show that for any $\delta > 0$ and $\gamma \in (0,1)$, there exists a constant $C_1' \geq 1$ such that for sufficiently large $n$,

$$\sup_{i,j<p_n, i\neq j, r\leq m_n} \mathbb{P}(|\tilde{\theta}_{ip_n}^{(i,j)}(\mathcal{G}_{nr}) - \theta_{ip_n}^{(i,j)}(\mathcal{G}_{nr})| > \delta) \leq 8\exp(-C_1' n^\gamma).$$

By choosing $\gamma \in (1-b, 1)$ (see assumption (A3)), the proof then follows analogously to the proof of Theorem 6.1 of the main text. □

LEMMA 17.1. *Assume that (A1), (A3) and (A5′) hold. Then for any $\delta > 0$ and $\gamma \in (0,1)$, there exists a constant $N > 0$ depending on $\delta$ and $v'$ (see assumption (A5′)), such that for all $n \geq N^{1/b(1-\gamma)}$,*

$$\sup_{i,j<p_n, i\neq j, r\leq m_n} \mathbb{P}(|\tilde{\theta}_{ip_n}^{(i,j)}(\mathcal{G}_{nr}) - \theta_{ip_n}^{(i,j)}(\mathcal{G}_{nr})| > \delta) \leq 8\exp(-C_1' n^\gamma),$$

*where $C_1'$ is a constant depending on $\gamma$ and $b$ is given in assumption (A3).*

PROOF. It is sufficient to prove that for any $i, j < p_n$, $i \neq j$ and any $r \leq m_n$,

$$\mathbb{P}(|\tilde{\theta}_{ip_n}^{(i,j)}(\mathcal{G}_{nr}) - \theta_{ip_n}^{(i,j)}(\mathcal{G}_{nr})| > \delta) \leq 8\exp(-C_1' n^\gamma) \quad \forall n \geq N^{1/b(1-\gamma)},$$

where the constants $C_1'$ and $N$ do not depend on the choice of $i, j$ and $r$.

Thus, we fix $i, j$ and $r$ and for notational convenience we denote the covariance matrix of $\mathbf{U}_{nijr} := \{X_{ni}, X_{nj}, X_{np_n}\} \cup \mathbf{PA}_i(\mathcal{G}_{nr}) \cup \mathbf{PA}_j(\mathcal{G}_{nr})$ and $\mathbf{U}_{nijr}(\mathcal{G}_{nr}) \setminus \{X_{np_n}\}$ by $\Sigma$ and $\Sigma'$ respectively. Let $\hat{\Sigma}$ denote the sample covariance matrix that corresponds to $\Sigma$. Let $\Sigma^{(i,j)}$ and $\hat{\Sigma}^{(i,j)}$ be the output of Algorithm 3.1 of the main text, applied to $\Sigma$ and $\hat{\Sigma}$ with intervention variables $(X_{ni}, X_{nj})$. We write $\Sigma'^{-1}$ and $\Sigma^{(i,j)-1}$ to denote $(\Sigma')^{-1}$ and $(\Sigma^{(i,j)})^{-1}$.

We assume $X_{np_n} \notin \mathbf{PA}_i(\mathcal{G}_{nr})$, since otherwise $\tilde{\theta}_{ip_n}^{(i,j)}(\mathcal{G}_{nr}) = \theta_{ip_n}^{(i,j)}(\mathcal{G}_{nr}) = 0$. Thus, we have

$$\tilde{\theta}_{ip_n}^{(i,j)}(\mathcal{G}_{nr}) = \frac{\hat{\Sigma}_{x_{ni}x_{np_n}}^{(i,j)}}{\hat{\Sigma}_{x_{ni}x_{ni}}^{(i,j)}} \quad \text{and} \quad \theta_{ip_n}^{(i,j)}(\mathcal{G}_{nr}) = \frac{\Sigma_{x_{ni}x_{np_n}}^{(i,j)}}{\Sigma_{x_{ni}x_{ni}}^{(i,j)}}.$$

By applying the inequality $|b_n|\ |a_n/b_n - a/b| \leq\ |a_n - a| + |b_n - b|\ |a|/|b|$, we obtain

$$\begin{aligned} &\hat{\Sigma}_{x_{ni}x_{ni}}^{(i,j)} \left|\tilde{\theta}_{ip_n}^{(i,j)}(\mathcal{G}_{nr}) - \theta_{ip_n}^{(i,j)}(\mathcal{G}_{nr})\right| \\ &\leq \left|\hat{\Sigma}_{x_{ni}x_{np_n}}^{(i,j)} - \Sigma_{x_{ni}x_{np_n}}^{(i,j)}\right| + \frac{|\Sigma_{x_{ni}x_{np_n}}^{(i,j)}|}{\Sigma_{x_{ni}x_{ni}}^{(i,j)}} \left|\hat{\Sigma}_{x_{ni}x_{ni}}^{(i,j)} - \Sigma_{x_{ni}x_{ni}}^{(i,j)}\right|. \end{aligned} \tag{4}$$

Note that $\Sigma^{(i,j)}_{x_{ni}x_{ni}} = \Sigma'^{(i,j)}_{x_{ni}x_{ni}}$ and

$$1/\Sigma'^{(i,j)}_{x_{ni}x_{ni}} \leq ||\Sigma'^{(i,j)-1}|| \leq M_2||\Sigma'^{-1}|| \leq M_2 v'/||\Sigma||, \tag{5}$$

where $M_2$ is a constant depending on $v'$. Here the first inequality follows from Cauchy interlacing theorem (which states that the eigenvalues of a Hermitian matrix $A$ of order $r$ are interlaced with those of any principal submatrix of order $r-1$), the second inequality follows from Lemma 17.2 (see below), and the last inequality follows from assumption (A5$'$). Hence,

$$\frac{|\Sigma^{(i,j)}_{x_{ni}x_{np_n}}|}{\Sigma^{(i,j)}_{x_{ni}x_{ni}}} \leq \frac{M_2 v'|\Sigma^{(i,j)}_{x_{ni}x_{np_n}}|}{||\Sigma||} \leq \frac{M_2 v'||\Sigma^{(i,j)}||}{||\Sigma||} \leq M_2^2 v',$$

where the second inequality follows since $||A||_{\max} = \max_{i,j}|A_{ij}| \leq ||A||$ for any matrix $A$, and the last inequality follows from Lemma 17.2.

Define $B_{ij} := \{\hat{\Sigma}'^{(i,j)}_{x_{ni}x_{ni}} \geq \frac{1}{2}\Sigma'^{(i,j)}_{x_{ni}x_{ni}}\}$. Since $||\hat{\Sigma}^{(i,j)} - \Sigma^{(i,j)}||_{\max} \leq ||\hat{\Sigma}^{(i,j)} - \Sigma^{(i,j)}||$ and $\hat{\Sigma}^{(i,j)}_{x_{ni}x_{ni}} = \hat{\Sigma}'^{(i,j)}_{x_{ni}x_{ni}}$, we have the following inequality on the set $B_{ij}$:

$$\left|\tilde{\theta}^{(i,j)}_{ip_n}(\mathcal{G}_{nr}) - \theta^{(i,j)}_{ip_n}(\mathcal{G}_{nr})\right| \leq \frac{2(1+M_2^2 v')}{\Sigma'^{(i,j)}_{x_{ni}x_{ni}}}||\hat{\Sigma}^{(i,j)} - \Sigma^{(i,j)}||.$$

Therefore, from (5) and assumption (A5$'$), it follows that there exists a constant $C_4$ depending on $v'$ such that on the set $B_{ij}$, we have

$$\left|\tilde{\theta}^{(i,j)}_{ip_n}(\mathcal{G}_{nr}) - \theta^{(i,j)}_{ip_n}(\mathcal{G}_{nr})\right| \leq \frac{C_4}{||\Sigma||}||\hat{\Sigma}^{(i,j)} - \Sigma^{(i,j)}||.$$

This implies

$$\mathbb{P}\left(\left|\tilde{\theta}^{(i,j)}_{ip_n}(\mathcal{G}_{nr}) - \theta^{(i,j)}_{ip_n}(\mathcal{G}_{nr})\right| > \delta\right) \leq \mathbb{P}\left(||\hat{\Sigma}^{(i,j)} - \Sigma^{(i,j)}|| > \delta||\Sigma||/C_4\right) + P(B^C_{ij}).$$

By Lemma 17.3 (see below) there exists a constant $N$ depending on $\delta$ and $v'$, such that for $n \geq N^{1/b(1-\gamma)}$ the first term is bounded by $4\exp(-C_2' n^{\gamma})$, where $C_2'$ depends only on $\gamma$. Furthermore, note that

$$B_{ij} \supseteq \{|\hat{\Sigma}'^{(i,j)}_{x_{ni}x_{ni}} - \Sigma'^{(i,j)}_{x_{ni}x_{ni}}| \leq \Sigma'^{(i,j)}_{x_{ni}x_{ni}}/2\} \supseteq \{||\hat{\Sigma}^{(i,j)} - \Sigma^{(i,j)}|| \leq ||\Sigma||/(2M_2 v')\}.$$

Therefore, again from Lemma 17.3, we have, $P(B^C_{ij}) \leq 4\exp(-C_2' n^{\gamma})$, for all $n \geq N'^{1/b(1-\gamma)}$, where $N'$ is a constant depending on $v'$. This completes the proof since the constants $C_2'$, $N$ and $N'$ do not depend on the choice of $i$,$j$ and $r$. $\square$

The following lemma shows that the operation of modifying a covariance matrix through Algorithm 3.1 of the main text is a Lipschitz continuous function, where the Lipschitz constant depends only on $v'$ (see assumption (A5$'$)). We will use this result to prove Lemma 17.3.

LEMMA 17.2. *Let $\Sigma$, $\hat{\Sigma}$, $\Sigma^{(i,j)}$ and $\hat{\Sigma}^{(i,j)}$ be as in the proof of Lemma 17.1. Let $\Sigma^{(i)}$ and $\hat{\Sigma}^{(i)}$ be the output of Algorithm 3.1 of the main text, applied to $\Sigma$ and $\hat{\Sigma}$ with the intervention variable $X_{ni}$. Under assumption (A5$'$), there exist constants $M_1$, $M_2$ and $K_1$ depending only on $v'$ such that the following inequalities hold:*

1. $||\Sigma^{(i)}|| \leq M_1||\Sigma||$ *and* $||\Sigma'^{(i)-1}|| \leq M_1||\Sigma'^{-1}||$;
2. $||\Sigma^{(i,j)}|| \leq M_2||\Sigma||$ *and* $||\Sigma'^{(i,j)-1}|| \leq M_2||\Sigma'^{-1}||$;
3. *on the set* $B := \{||\hat{\Sigma}-\Sigma|| \leq 1/(2||\Sigma'^{-1}||)\}$, $||\hat{\Sigma}^{(i)}-\Sigma^{(i)}|| \leq K_1\, ||\hat{\Sigma}-\Sigma||$.

PROOF. Let $\mathbf{Z} := \mathbf{PA}_i(\mathcal{G}_{nr}) \cup \{X_{ni}\}$ and $\mathbf{W} = \mathbf{U}_{nijr} \setminus \mathbf{Z}$. Without loss of generality, we assume that variables in $\Sigma$ and $\Sigma^{(i)}$ are ordered as $(\mathbf{Z}, \mathbf{W})$.

Recall from Corollary 8.2 that $\Sigma^{(i)} = Q^{(i)}\Sigma$, where

$$Q^{(i)} = \begin{pmatrix} \Sigma^{(i)}_{\mathbf{zz}}\Sigma^{-1}_{\mathbf{zz}} & \mathbf{0} \\ \Sigma_{\mathbf{wz}}\Sigma^{-1}_{\mathbf{zz}}(\Sigma^{(i)}_{\mathbf{zz}}\Sigma^{-1}_{\mathbf{zz}} - \mathrm{I}) & \mathrm{I} \end{pmatrix} \text{ with } \Sigma^{(i)}_{\mathbf{zz}} = \begin{pmatrix} \Sigma_{\mathbf{pa}_i\mathbf{pa}_i} & \mathbf{0} \\ \mathbf{0} & \Sigma_{\mathbf{zz}}/\Sigma_{\mathbf{pa}_i\mathbf{pa}_i} \end{pmatrix},$$

where $\Sigma_{\mathbf{zz}}/\Sigma_{\mathbf{pa}_i\mathbf{pa}_i} := \Sigma_{x_{ni}x_{ni}} - \Sigma_{x_{ni}\mathbf{pa}_i}\Sigma^{-1}_{\mathbf{pa}_i\mathbf{pa}_i}\Sigma_{\mathbf{pa}_i x_{ni}}$, is the Schur complement of $\Sigma_{\mathbf{pa}_i\mathbf{pa}_i}$ in $\Sigma_{\mathbf{zz}}$.

Therefore, to complete the proof of statement 1, it is enough to show that there exists a constant $M_1$ depending only on $v'$ such that $||Q^{(i)}|| \leq M_1$ and $||Q^{(i)-1}|| \leq M_1$. From the standard properties of the spectral norm it follows that

$$||Q^{(i)}|| \leq ||\Sigma^{(i)}_{\mathbf{zz}}||\ ||\Sigma^{-1}_{\mathbf{zz}}|| + ||\Sigma_{\mathbf{wz}}||\ ||\Sigma^{-1}_{\mathbf{zz}}||\ ||\Sigma^{(i)}_{\mathbf{zz}}\Sigma^{-1}_{\mathbf{zz}} - \mathrm{I}|| + ||\mathrm{I}||.$$

Thus, to prove $||Q^{(i)}|| \leq M_1$, it suffices to show that both $||\Sigma^{(i)}_{\mathbf{zz}}||\ ||\Sigma^{-1}_{\mathbf{zz}}||$ and $||\Sigma_{\mathbf{wz}}||\ ||\Sigma^{-1}_{\mathbf{zz}}||$ are bounded, since $||\mathrm{I}|| = 1$ and $||\Sigma^{(i)}_{\mathbf{zz}}\Sigma^{-1}_{\mathbf{zz}} - \mathrm{I}|| \leq ||\Sigma^{(i)}_{\mathbf{zz}}||\ ||\Sigma^{-1}_{\mathbf{zz}}|| + 1$. Hence, the result follows from the following inequalities and assumption (A5$'$):

(i) $||\Sigma^{(i)}_{\mathbf{zz}}|| \leq \max(||\Sigma_{\mathbf{pa}_i\mathbf{pa}_i}||,\ \Sigma_{x_{ni}x_{ni}}) \leq ||\Sigma_{\mathbf{zz}}||$;
(ii) $||\Sigma_{\mathbf{wz}}|| \leq ||\Sigma_{\mathbf{zz}}||^{1/2}\ ||\Sigma_{\mathbf{ww}}||^{1/2}$;
(iii) $||\Sigma_{\mathbf{zz}}|| \leq ||\Sigma||$ and $||\Sigma_{\mathbf{ww}}|| \leq ||\Sigma||$;
(iv) $||\Sigma^{-1}_{\mathbf{zz}}|| \leq ||\Sigma'^{-1}||$.

The first inequality of (i) follows from $0 \leq \Sigma_{\mathbf{zz}}/\Sigma_{\mathbf{pa}_i\mathbf{pa}_i} \leq \Sigma_{x_{ni}x_{ni}}$. The second inequality of (i) follows from Cauchy interlacing theorem, and so do (iii) and (iv). Finally, (ii) is simply Cauchy-Schwarz.

The proof of $||Q^{(i)-1}|| \leq M_1$ is similar, since

$$Q^{(i)-1} = \begin{pmatrix} \Sigma_{\mathbf{zz}}\Sigma_{\mathbf{zz}}^{(i)-1} & \mathbf{0} \\ \Sigma_{\mathbf{wz}}\Sigma_{\mathbf{zz}}^{-1}(\Sigma_{\mathbf{zz}}\Sigma_{\mathbf{zz}}^{(i)-1} - \mathrm{I}) & \mathrm{I} \end{pmatrix}$$

and

$$||\Sigma_{\mathbf{zz}}^{(i)-1}|| \leq 1/\min(\lambda_{\min}(\Sigma_{\mathbf{pa}_i\mathbf{pa}_i}),\ \Sigma_{\mathbf{zz}}/\Sigma_{\mathbf{pa}_i\mathbf{pa}_i}) \leq 1/\lambda_{\min}(\Sigma_{\mathbf{zz}}) = ||\Sigma_{\mathbf{zz}}^{-1}||.$$

The last inequality follows from the interlacing property of eigenvalues of a Hermitian $A$ and eigenvalues of the Schur complement of any principal submatrix of $A$ (see, for example, Corollary 2.3 of [25]).

Note that statement 1 and assumption (A5$'$) assure that $||\Sigma^{(i)}||\ ||\Sigma^{(i)\prime-1}|| \leq M_1^2 v'$. Thus, by the same argument as in the proof of statement 1, we have $||\Sigma^{(i,j)}|| \leq M_1'||\Sigma^{(i)}||$ and $||\Sigma'^{(i,j)-1}|| \leq M_1'||\Sigma'^{(i)-1}||$, for some constant $M_1'$ depending on $v'$. Hence, statement 2 follows from statement 1.

Now we prove statement 3. Let $\hat{\Sigma}^{(i)}$ and $\hat{Q}^{(i)}$ be the sample analogue of $\Sigma^{(i)}$ and $Q^{(i)}$ respectively. Thus, we have, $\hat{\Sigma}^{(i)} = \hat{Q}^{(i)}\hat{\Sigma}$. Using the triangle inequality and the submultiplicity property of the spectral norm, we obtain

$$\begin{aligned} &||\hat{\Sigma}^{(i)} - \Sigma^{(i)}|| \\ &\leq ||\hat{Q}^{(i)} - Q^{(i)}||\ ||\hat{\Sigma} - \Sigma|| + \ ||Q^{(i)}||\ ||\hat{\Sigma} - \Sigma||\ + ||\hat{Q}^{(i)} - Q^{(i)}||\ ||\Sigma||. \end{aligned} \tag{6}$$

The second term of (6) is bounded above by $M_1||\hat{\Sigma} - \Sigma||$, since we have shown that $||Q^{(i)}|| \leq M_1$. To bound the first and the third term, we will show that on the set $B$, there exists a positive constant $K_1'$ depending only on $v'$ such that $||\hat{Q}^{(i)} - Q^{(i)}|| \leq K_1'\ ||\Sigma'^{-1}||\ ||\hat{\Sigma} - \Sigma||$. This immediately implies on the set $B$, $||\hat{Q}^{(i)} - Q^{(i)}|| \leq K_1'/2$, since $||\hat{\Sigma} - \Sigma|| \leq 1/(2||\Sigma'^{-1}||)$. Hence, the first term of (6) is bounded above by $(K_1'/2)||\hat{\Sigma} - \Sigma||$ and the third term of (6) is bounded by $K_1'\ ||\Sigma'^{-1}||\ ||\hat{\Sigma} - \Sigma||\ ||\Sigma|| \leq (K_1'v')\ ||\hat{\Sigma} - \Sigma||$.

We now complete the proof by showing $||\hat{Q}^{(i)} - Q^{(i)}|| \leq K_1'\ ||\Sigma'^{-1}||\ ||\hat{\Sigma} - \Sigma||$. Some elementary calculations lead to the following inequalities:

$$\begin{aligned} &||\hat{Q}^{(i)} - Q^{(i)}|| \\ &\leq ||\hat{\Sigma}_{\mathbf{zz}}^{(i)}\hat{\Sigma}_{\mathbf{zz}}^{-1} - \Sigma_{\mathbf{zz}}^{(i)}\Sigma_{\mathbf{zz}}^{-1}|| + ||\hat{\Sigma}_{\mathbf{wz}}\hat{\Sigma}_{\mathbf{zz}}^{-1}(\hat{\Sigma}_{\mathbf{zz}}^{(i)}\hat{\Sigma}_{\mathbf{zz}}^{-1} - \mathrm{I}) - \Sigma_{\mathbf{wz}}\Sigma_{\mathbf{zz}}^{-1}(\Sigma_{\mathbf{zz}}^{(i)}\Sigma_{\mathbf{zz}}^{-1} - \mathrm{I})|| \\ &\leq 2||\hat{\Sigma}_{\mathbf{zz}}^{(i)}\hat{\Sigma}_{\mathbf{zz}}^{-1} - \Sigma_{\mathbf{zz}}^{(i)}\Sigma_{\mathbf{zz}}^{-1}|| + ||\hat{\Sigma}_{\mathbf{wz}}\hat{\Sigma}_{\mathbf{zz}}^{-1} - \Sigma_{\mathbf{wz}}\Sigma_{\mathbf{zz}}^{-1}||\ ||\hat{\Sigma}_{\mathbf{zz}}^{(i)}\hat{\Sigma}_{\mathbf{zz}}^{-1} - \Sigma_{\mathbf{zz}}^{(i)}\Sigma_{\mathbf{zz}}^{-1}|| \\ &\quad + ||\Sigma_{\mathbf{zz}}^{(i)}||\ ||\Sigma_{\mathbf{zz}}^{-1}||\ ||\hat{\Sigma}_{\mathbf{wz}}\hat{\Sigma}_{\mathbf{zz}}^{-1} - \Sigma_{\mathbf{wz}}\Sigma_{\mathbf{zz}}^{-1}|| + ||\Sigma_{\mathbf{wz}}||\ ||\Sigma_{\mathbf{zz}}^{-1}||\ ||\hat{\Sigma}_{\mathbf{zz}}^{(i)}\hat{\Sigma}_{\mathbf{zz}}^{-1} - \Sigma_{\mathbf{zz}}^{(i)}\Sigma_{\mathbf{zz}}^{-1}||. \end{aligned}$$

Since we have shown that both $||\Sigma^{(i)}_{\mathbf{zz}}||\ ||\Sigma^{-1}_{\mathbf{zz}}||$ and $||\Sigma_{\mathbf{wz}}||\ ||\Sigma^{-1}_{\mathbf{zz}}||$ are bounded above by constants depending on $v'$, it suffices to show that on the set $B$, there exist positive constants $K_2$ and $K_3$ such that

$$||\hat{\Sigma}_{\mathbf{wz}}\hat{\Sigma}^{-1}_{\mathbf{zz}} - \Sigma_{\mathbf{wz}}\Sigma^{-1}_{\mathbf{zz}}|| \le K_2\ ||\Sigma'^{-1}||\ ||\hat{\Sigma} - \Sigma|| \tag{7}$$

and

$$||\hat{\Sigma}^{(i)}_{\mathbf{zz}}\hat{\Sigma}^{-1}_{\mathbf{zz}} - \Sigma^{(i)}_{\mathbf{zz}}\Sigma^{-1}_{\mathbf{zz}}|| \le K_3\ ||\Sigma'^{-1}||\ ||\hat{\Sigma} - \Sigma||. \tag{8}$$

Again, applying the triangle inequality and the submultiplicity property of the spectral norm, it is easy to check that the left hand side of (7) satisfies the following inequality:

$$\begin{aligned} &||\hat{\Sigma}_{\mathbf{wz}}\hat{\Sigma}^{-1}_{\mathbf{zz}} - \Sigma_{\mathbf{wz}}\Sigma^{-1}_{\mathbf{zz}}|| \\ \le\ & ||\hat{\Sigma}_{\mathbf{wz}} - \Sigma_{\mathbf{wz}}||\ ||\hat{\Sigma}^{-1}_{\mathbf{zz}} - \Sigma^{-1}_{\mathbf{zz}}|| + ||\Sigma^{-1}_{\mathbf{zz}}||\ ||\hat{\Sigma}_{\mathbf{wz}} - \Sigma_{\mathbf{wz}}|| + ||\Sigma_{\mathbf{wz}}||\ ||\hat{\Sigma}^{-1}_{\mathbf{zz}} - \Sigma^{-1}_{\mathbf{zz}}|| \\ \le\ & ||\hat{\Sigma} - \Sigma||\ ||\hat{\Sigma}^{-1}_{\mathbf{zz}} - \Sigma^{-1}_{\mathbf{zz}}|| + ||\Sigma'^{-1}||\ ||\hat{\Sigma} - \Sigma|| + ||\Sigma||\ ||\hat{\Sigma}^{-1}_{\mathbf{zz}} - \Sigma^{-1}_{\mathbf{zz}}||. \end{aligned} \tag{9}$$

We now show that (7) follows from (9) and assumption (A5′), since on the set $B$, we have $||\hat{\Sigma}^{-1}_{\mathbf{zz}} - \Sigma^{-1}_{\mathbf{zz}}|| \le 2||\Sigma'^{-1}||^2\ ||\Sigma - \hat{\Sigma}||$. To see this, we first write $\hat{\Sigma}^{-1}_{\mathbf{zz}} = \Sigma^{-1}_{\mathbf{zz}}(\mathrm{I} - \Sigma^{-1}_{\mathbf{zz}}(\Sigma_{\mathbf{zz}} - \hat{\Sigma}_{\mathbf{zz}}))^{-1}$ to obtain that on the set $B$

$$||\hat{\Sigma}^{-1}_{\mathbf{zz}}|| \le ||\Sigma^{-1}_{\mathbf{zz}}||\ ||(\mathrm{I} - \Sigma^{-1}_{\mathbf{zz}}(\Sigma_{\mathbf{zz}} - \hat{\Sigma}_{\mathbf{zz}}))^{-1}|| \le \frac{||\Sigma^{-1}_{\mathbf{zz}}||}{1 - ||\Sigma^{-1}_{\mathbf{zz}}(\Sigma_{\mathbf{zz}} - \hat{\Sigma}_{\mathbf{zz}})||} \le 2||\Sigma^{-1}_{\mathbf{zz}}||. \tag{10}$$

Note that the second inequality requires $||\Sigma^{-1}_{\mathbf{zz}}(\Sigma_{\mathbf{zz}} - \hat{\Sigma}_{\mathbf{zz}})|| < 1$ and this holds on the set $B$, since $||\Sigma^{-1}_{\mathbf{zz}}(\Sigma_{\mathbf{zz}} - \hat{\Sigma}_{\mathbf{zz}})|| \le ||\Sigma^{-1}_{\mathbf{zz}}||\ ||\Sigma_{\mathbf{zz}} - \hat{\Sigma}_{\mathbf{zz}}|| \le ||\Sigma'^{-1}||\ ||\Sigma - \hat{\Sigma}|| \le 1/2$.

Next, we write $(\hat{\Sigma}^{-1}_{\mathbf{zz}} - \Sigma^{-1}_{\mathbf{zz}}) = \hat{\Sigma}^{-1}_{\mathbf{zz}}(\Sigma_{\mathbf{zz}} - \hat{\Sigma}_{\mathbf{zz}})\Sigma^{-1}_{\mathbf{zz}}$ and then apply the submultiplicity property of the spectral norm and (10), to obtain that on the set $B$

$$||\hat{\Sigma}^{-1}_{\mathbf{zz}} - \Sigma^{-1}_{\mathbf{zz}}|| \le 2||\Sigma^{-1}_{\mathbf{zz}}||^2\ ||\Sigma_{\mathbf{zz}} - \hat{\Sigma}_{\mathbf{zz}}|| \le 2||\Sigma'^{-1}||^2\ ||\Sigma - \hat{\Sigma}||.$$

This completes the proof of (7).

Using similar techniques, it can be shown that on the set $B$ we have $||\hat{\Sigma}^{(i)}_{\mathbf{zz}} - \Sigma^{(i)}_{\mathbf{zz}}|| \le K_4||\hat{\Sigma} - \Sigma||$, for some constant $K_4$ depending only on $v'$. Hence, we can conclude (8), using a proof that is analogous to the one of (7). □

LEMMA 17.3. *Assume that (A1), (A3) and (A5′) hold. Let $\Sigma$, $\hat{\Sigma}$, $\Sigma^{(i,j)}$ and $\hat{\Sigma}^{(i,j)}$ be as in the proof of Lemma 17.1. Then for any $\delta > 0$ and $\gamma \in (0,1)$, there exists a constant $N > 0$ depending only on $\delta$ and $v'$ such that for all $n \geq N^{1/b(1-\gamma)}$,*

$$\mathbb{P}\left(||\hat{\Sigma}^{(i,j)} - \Sigma^{(i,j)}|| > \delta||\Sigma||\right) \leq 4\exp\left(-C_2' n^{\gamma}\right),$$

*where $C_2' \geq 1$ is a constant depending only on $\gamma$.*

PROOF. Let $q_n' \times q_n'$ be the dimension $\Sigma$. The Gaussian assumption assures that for any $\delta \in (0,1)$ and $t \geq 1$, the following holds with probability at least $1 - 2\exp(-t^2 q_n')$ (see page 31 of [24]):

$$\text{If } n \geq C'(t/\delta)^2 q_n' \text{ then } ||\hat{\Sigma} - \Sigma|| \leq \delta||\Sigma||,$$

where $C'$ is a pure constant. We choose $t^2 = (n/q_n')^{\gamma}$ to obtain

$$\mathbb{P}(||\hat{\Sigma} - \Sigma|| > \delta||\Sigma||) \leq 2\exp\left(-n^{\gamma} q_n'^{1-\gamma}\right) \quad \text{for } \left(\frac{n}{q_n'}\right)^{1-\gamma} \geq \frac{C'}{\delta^2}.$$

Now since $3 \leq q_n' \leq 2q_n + 3 = \mathcal{O}(n^{1-b})$, for $C_2' = 3^{1-\gamma}$ and some constant $C_3'$ depending on $\gamma$ the following holds.

$$\mathbb{P}(||\hat{\Sigma} - \Sigma|| > \delta||\Sigma||) \leq 2\exp\left(-C_2' n^{\gamma}\right) \quad \text{for } n^{b(1-\gamma)} \geq \frac{C_3'}{\delta^2}. \tag{11}$$

Let $\Sigma^{(i)}$ and $\hat{\Sigma}^{(i)}$ be as in Lemma 17.2. Note that the proof of Lemma 17.2 only requires the assumption $||\Sigma||\ ||\Sigma'^{-1}||$ is bounded. Now the first part of Lemma 17.2 assures that $||\Sigma^{(i)}||\ ||\Sigma^{(i)\prime-1}|| \leq M_1^2 v'$. Thus Lemma 17.2 implies that there exists a constant $K_2 > 0$ such that on the set $B_i := \{||\hat{\Sigma}^{(i)} - \Sigma^{(i)}|| \leq 1/(2||\Sigma'^{(i)-1}||)\}$, $||\hat{\Sigma}^{(i,j)} - \Sigma^{(i,j)}|| \leq K_2\ ||\hat{\Sigma}^{(i)} - \Sigma^{(i)}||$.

Let $B$ be as in Lemma 17.2. Then on the set $B \cap B_i$,

$$||\hat{\Sigma}^{(i,j)} - \Sigma^{(i,j)}|| \leq K_1 K_2\ ||\hat{\Sigma} - \Sigma||,$$

Therefore,

$$\mathbb{P}\left(||\hat{\Sigma}^{(i,j)} - \Sigma^{(i,j)}|| > \delta||\Sigma||\right) \leq \mathbb{P}\left(||\hat{\Sigma} - \Sigma|| > \delta||\Sigma||/(K_1K_2)\right) + \mathbb{P}((B \cap B_i)^C). \tag{12}$$

For any $\gamma \in (0,1)$, (11) assures that there exists $N > 0$ depending on $\delta$ and $v'$, such that the first term of (12) is bounded by $2\exp(-C_2' n^{\gamma})$ for all

$n \geq N^{1/b(1-\gamma)}$. We complete the proof by showing the same for the second term of (12).

Let $B' := \{||\hat{\Sigma} - \Sigma|| \leq 1/(2K_3||\Sigma'^{-1}||)\}$, where $K_3 = \max(K_1M_1, 1)$. Then $B' \subseteq B$ since $K_3 > 1$ and hence $B' \subseteq B_i$, since Lemma 17.2 implies that on the set $B'$

$$||\hat{\Sigma}^{(i)} - \Sigma^{(i)}|| \leq K_1||\hat{\Sigma} - \Sigma|| \leq \frac{K_1}{2K_3||\Sigma'^{-1}||} \leq \frac{K_1M_1}{2K_3||\Sigma'^{(i)-1}||} \leq \frac{1}{2||\Sigma'^{(i)-1}||}.$$

Thus $\mathbb{P}((B \cap B_i)^C) \leq \mathbb{P}(B'^c)$ and putting $1/\delta = 2K_3\ ||\Sigma'^{-1}||\ ||\Sigma||$ in (11) gives, for $n^{b(1-\gamma)} \geq N'$,

$$\mathbb{P}(B'^C) = \mathbb{P}(||\hat{\Sigma} - \Sigma|| > 1/(2K_3||\Sigma'^{-1}||)) \leq 2\exp(-C_2'n^\gamma),$$

where $N'$ is a constant depending on $v'$. □

**18. Simulations in sparse high-dimensional settings with Gaussian errors.** In this section we provide empirical support for Corollary 6.1 of the main text. Moreover, we empirically compare the performances of the joint-IDA estimators based on RRC, MCD and IPW.

We randomly simulate $n_{iter} = 5000$ Gaussian linear SEMs as in Section 14, with $p = 1000$, where we impose a special block structure of 100 connected components of size 10 with $ens = 2$. In each iteration, a pair of intervention nodes $\{X_{i_t}^{(t)}, X_{j_t}^{(t)}\}$ and a response variable $X_{r_t}^{(t)}$ are chosen as before, but we restrict them to belong to one of the 100 disconnected blocks (randomly chosen) since otherwise the total joint effect can be easily identified as zero.

We generate standardized data using the true correlation matrix as in Section 14, for 6 different sample sizes: $n_{sample} = 50, 100, 200, 400, 800, 1600$. We estimate the CPDAG using the order independent version of the PC-algorithm with tuning parameter $\alpha = 0.01$.

For $t = 1, \ldots, n_{iter}$ and $\ell = i_t, j_t$, we compute the errors for estimating $\text{minabs}(\Theta_{\ell r_t}^{(i_t,j_t)}(\mathcal{C}^{(t)}))$ and $\text{aver}(\Theta_{\ell r_t}^{(i_t,j_t)}(\mathcal{C}^{(t)}))$ using the joint-IDA estimators based on RRC, MCD and IPW. Figure 10 shows log-log plots of the mean absolute error (MAE) for the cases where $\text{minabs}(\Theta_{\ell r_t}^{(i_t,j_t)}(\mathcal{C}^{(t)})) < 0.1$ or $|\text{aver}(\Theta_{\ell r_t}^{(i_t,j_t)}(\mathcal{C}^{(t)}))| < 0.1$, and the mean absolute relative error (MARE) for the other cases where the magnitudes of the corresponding summary measures are at least as large as 0.1. We again see that RRC and MCD outperform IPW. The difference between RRC and MCD on the one hand and IPW on the other hand becomes larger as the sample size increases. Moreover, the difference between IPW and RRC (or MCD) is more pronounced for zero and small effects, indicating that IPW is more prone to false positive results.

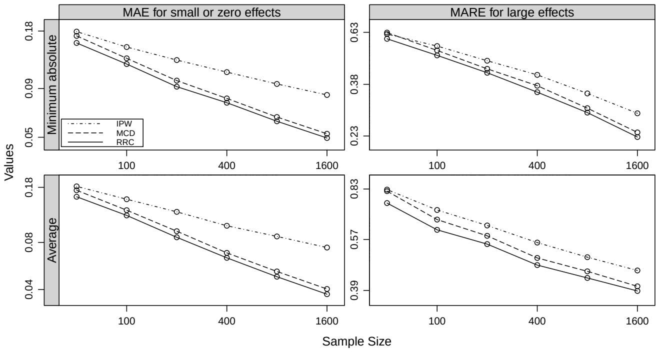


Fig 10: Log-log plot of the mean absolute error (MAE) for zero or small joint effects (left panel) and the mean absolute relative error (MARE) for large joint effects (right panel) against sample size, for estimating $\text{minabs}(\Theta_{\ell r_t}^{(i_t,j_t)}(\mathcal{C}^{(t)}))$ (upper panel) and $\text{aver}(\Theta_{\ell r_t}^{(i_t,j_t)}(\mathcal{C}^{(t)}))$ (lower panel) for $\ell = i_t, j_t$ and $t = 1, \ldots, n_{iter}$. (Cf. Corollary 6.1 of the main text.)

**19. Application of the joint-IDA estimators on DREAM4 data.** The DREAM4 In Silico Network Challenge [12, 19] is a competition in reverse engineering of gene regulation networks, involving five networks of size 100. We will use these to test our joint-IDA methods.

Since the challenge does not contain i.i.d. observational data, we use as "observational data" steady state expression levels from 100 (in silico) single-gene knockout experiments, ignoring the knockout information. The challenge also contains steady state expression levels of all genes from 20 (in silico) different double-gene knockout experiments. We will use these values to validate our methods.

For each network, we denote the $(i, j)$-th entry of the $100 \times 100$ observational data matrix by $a_{ij}$, i.e., $a_{ij}$ is the steady state expression level of gene $j$ for observation $i$. We denote the average expression level of gene $j$ by $a_{\cdot j} = (\sum_{i=1}^{100} a_{ij})/100$. Similarly, for each network, we denote the $(i, j)$-th entry of the $20 \times 100$ gold standard data matrix by $b_{ij}$, i.e., $b_{ij}$ is the noise-free steady state expression level of gene $j$ in the $i$th double gene knockout experiment, where we let $(c_1(i), c_2(i))$ denote the pair of genes that is knocked out in the $i$th experiment. We denote the noise-free steady state expression level of gene $j$ by $w_j$.

First, we compute the gold-standard total increase in the expression value of gene $j$ due to knocking out the gene pair $(c_1(i), c_2(i))$ as

$$\Delta_{ij} = b_{ij} - w_j.$$

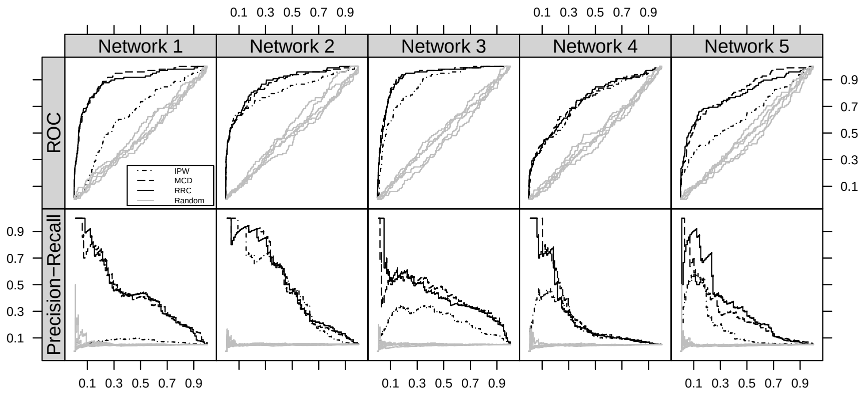


Fig 11: ROC curves (upper panel) and Precision-Recall curves (lower panel) for estimating the target set with top $r$ triples according to the large $|\bar{\Delta}_{ij}|$ values, $r = 1, \dots, 1960$. (DREAM4 data, see also Section 6 of the main text.)

For each network, we define our *target set* as the top 5% of $|\Delta_{ij}|$ values for the $20 \times 98$ triples $(c_1(i), c_2(i), j)$, $i = 1, \dots, 20$ and $j \in \{1, \dots, 100\} \setminus \{c_1(i), c_2(i)\}$.

To estimate the multisets of possible total joint effects (see Section 6 of the main text), we apply the joint-IDA estimator to the observational data, using intervention nodes $(c_1(i), c_2(i))$ and node of interest $j$, for $i = 1, \dots, 20$ and $j \in \{1, \dots, 100\} \setminus \{c_1(i), c_2(i)\}$. We use an order-independent modification [4] of the Rank-PC algorithm [6] (see Section 12 for details) with tuning parameter $\alpha = 0.05$, and OPIN methods RRC, MCD and IPW. We denote the resulting multiset of possible total joint effects by $\bar{\Theta}_j^{(c_1(i), c_2(i))}$ (as in Algorithm 6.1 of the main text), without specifying the OPIN method.

The gene expression levels of genes $c_1(i)$ and $c_2(i)$ are zero after knocking out the gene pair $(c_1(i), c_2(i))$. Hence, the decrease in the average gene expression levels of genes $c_1(i)$ and $c_2(i)$ due to the double knockout is given by $a_{.c_1(i)}$ and $a_{.c_2(i)}$, respectively. We combine (the average values of) the estimated multisets of possible total joint effects of genes $c_1(i)$ and $c_2(i)$ on gene j as follows:

$$\bar{\Delta}_{ij} = -a_{.c_1(i)} \operatorname{aver}(\bar{\Theta}_{c_1(i)j}^{(c_1(i), c_2(i))}) - a_{.c_2(i)} \operatorname{aver}(\bar{\Theta}_{c_2(i)j}^{(c_1(i), c_2(i))}),$$

where $\operatorname{aver}(A) := |A|^{-1} \sum_{a \in A} a$ for any multiset $A$.

For each network, we construct ROC and Precision-Recall curves for the target set based on the ordered values of $|\bar{\Delta}_{ij}|$ from RRC, MCD and IPW,

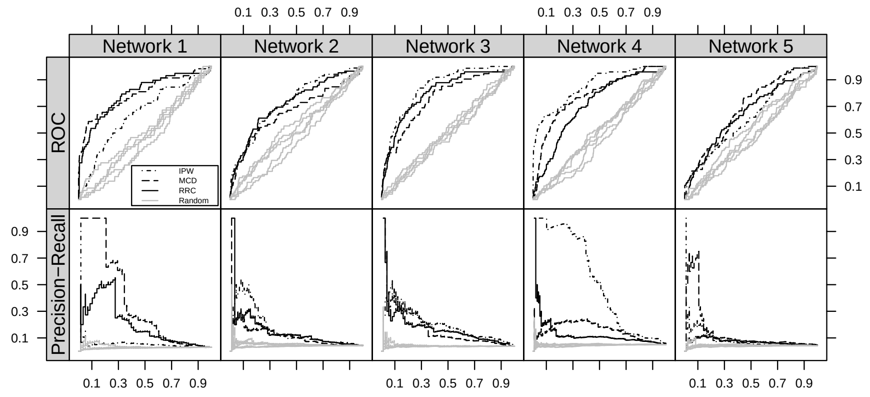


Fig 12: ROC curves (upper panel) and Precision-Recall curves (lower panel) for estimating the target set with top $r$ triples according to the large $|\bar{\Gamma}_{ij}|$ values, $r = 1, \dots, 1960$. (DREAM4 data, see also Section 6 of the main text.)

as well as from 5 random orderings. Figure 11 shows that both RRC and MCD perform significantly better than random guessing and outperform IPW. The differences in the performances between IPW and RRC/MCD are more apparent in the Precision-Recall curves.

Next, we look at the problem of estimating the strength of the epistatic interaction between a pair of genes [7, 22]. We compute the gold-standard difference between the effect of knocking out the gene pair $(c_1(i), c_2(i))$ and the sum of the effects of knocking out gene $c_1(i)$ and $c_2(i)$ separately as

$$\Gamma_{ij} = \Delta_{ij} - (a^*_{c_1(i)j} - w_j) - (a^*_{c_2(i)j} - w_j),$$

where $a^*_{rj}$ is the noise-free steady state expression level of gene $j$ when gene $r$ is knocked out. For each network, we define our *target set* as those triples $(c_1(i), c_2(i), j)$ for which $|\Gamma_{ij}| > 0.2$ (this corresponds to 2-5% of all values), $i = 1, \dots, 20$ and $j \in \{1, \dots, 100\} \setminus \{c_1(i), c_2(i)\}$.

We estimate $\Delta_{ij}$ by $\bar{\Delta}_{ij}$ as before and estimate $(a^*_{rj} - w_j)$ by $-a_{.r}\text{aver}(\bar{\Theta}_{rj})$ (using the estimated multiset of possible total effects of gene $r$ on gene $j$). Combining these, we obtain

$$\bar{\Gamma}_{ij} = \bar{\Delta}_{ij} + a_{.c_1(i)}\text{aver}(\bar{\Theta}_{c_1(i)j}) + a_{.c_2(i)}\text{aver}(\bar{\Theta}_{c_2(i)j}).$$

For each network, we construct ROC and Precision-Recall curves for the target set based on the ordered values of $|\bar{\Gamma}_{ij}|$ from RRC, MCD and IPW,

as well as from 5 random orderings. Figure 12 shows that all three method perform significantly better than random guessing and none of RRC, MCD or IPW outperforms the others.

Note that our main assumption that the data are generated from a linear SEM is not valid for the DREAM4 datasets (see [12, 19] for details about the data generating mechanism of these in-silico data). Using the given gold-standard networks, we can check whether the linearity assumption holds between a node and its parents, using Tukey-Anscombe (or residuals vs. fitted values) plots. Figure 13 shows Tukey-Anscombe plots for the 5 networks and 5 randomly chosen intervention variables regressed on their parents, where the intervention variables were chosen among the 20 overlapping pairs of intervention variables in the double-gene knockout experiments. We observe a slight violation of the linearity assumption in some cases. However, we still get informative results, in the sense that ROC and Precision-Recall curves of the joint-IDA estimators are much better than ROC and Precision-Recall curves of random guessing in Figures 11 and 12, suggesting that the methods are not very sensitive to small violations of linearity in this case.

Finally, we compare our joint-IDA estimators to an approach that simply takes empty parent sets for all intervention nodes. Figure 14 shows the ROC and Precision-Recall curves for estimating the target set that corresponds to Figure 11, but using empty parent sets. We see that, even with this naive assumption, ROC and Precision-Recall curves are still as good as in Figure 11. This phenomenon can happen in certain sparse networks (see Remark 3.1 of the main text and Remark 3.1 of this supplement). In Section 20, we show some examples where the jointIDA estimators do outperform this naive method.

If all parent sets are given to be empty, the estimates of the joint intervention effects would be identical to the corresponding estimates of the single intervention effects. Therefore, this naive method cannot be applied to estimate the target set that corresponds to large $|\Gamma_{ij}|$ values, since it would estimate all $\Gamma_{ij}$'s to be zero.

**20. Simulations in high-dimensional settings with non-Gaussian errors.** First, we randomly generate 5 weighted DAGs as in Section 14 but with $p = 1000$ vertices and expected neighborhood size $ens = 4$ (we call this "Scheme 1"). For each DAG, we simulate 1000 i.i.d. samples where we randomly choose each error variable to have either a standard normal distribution or a standardized Student's t-distribution with 3 degrees of freedom, each with probability 1/2.

We consider interesting triples of genes in the following way. We randomly

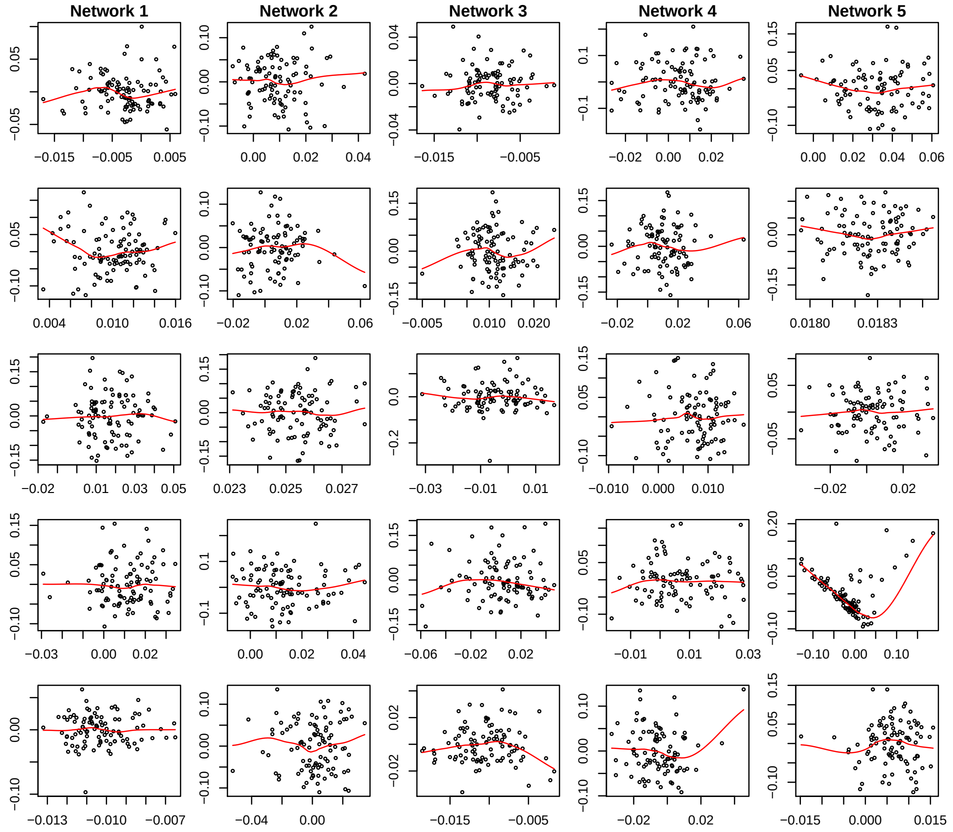


Fig 13: Tukey-Anscombe (or residuals vs. fitted values) plots for the DREAM4 data, for regressions of 5 randomly chosen intervention variables on their parents, after removing multivariate outliers based on Mahalanobis distance, for each of the five networks ($i$-th column corresponds to the $i$-th network). (See Section 19.)

choose 20 pairs of intervention variables for each DAG such that no intervention variable is an isolated node in the DAG. Then for each chosen pair of intervention variables $(X_i, X_j)$, we compute the total joint effect of $(X_i, X_j)$ on all other variables $X_k$ that are correlated with at least one of the two intervention variables. Finally, for each DAG, we choose the target set to be the set of all such triples $(i, j, k)$ for which $\theta_{ik}^{(i,j)}$ $(k \neq i, j)$ is non-zero (in each case the target set contains approximately 2.5%-5% of all triples ($\approx 10000$)).

To estimate $\theta_{ik}^{(i,j)}$, we apply the joint-IDA estimators (Algorithm 6.1 of

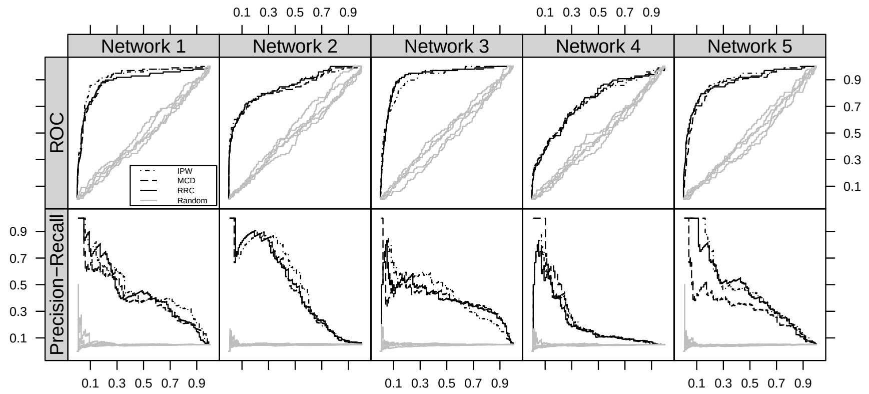


Fig 14: ROC curves (upper panel) and Precision-Recall curves (lower panel) for estimating the target set (that corresponds to top 5% $|\Delta_{ij}|$ values) with top $r$ triples ($r = 1, \dots, 1960$) according to the large $|\bar{\Delta}_{ij}|$ values, when assuming that the intervention variables have no parents. (DREAM4 data, see Section 19.)

the main text) on the simulated data, using intervention nodes $(i, j)$ and node of interest $k$. We use the order-independent version of the Rank-PC algorithm [4, 6, 20] with $\alpha = 0.01$, and OPIN methods RRC, MCD and IPW. We denote the resulting multiset of possible total joint effects by $\bar{\Theta}_{ik}^{(i,j)}$ (as in Algorithm 6.1 of the main text), without specifying the OPIN method. Finally, we obtain an estimate of $|\theta_{ik}^{(i,j)}|$ by computing absolute value of $\text{aver}(\bar{\Theta}_{ik}^{(i,j)})$, where $\text{aver}(A) := |A|^{-1} \sum_{a \in A} a$ for any multiset $A$.

For each network, we construct ROC and Precision-Recall curves for the target set based on the ordered values of $|\text{aver}(\bar{\Theta}_{ik}^{(i,j)})|$ from RRC, MCD and IPW, as well as from 5 different random orderings. Figure 15 shows that both RRC and MCD perform significantly better than random guessing and outperform IPW.

In Figure 16, we construct ROC and Precision-Recall curves in identical settings as in Figure 15, but assuming that the intervention variables have no parents. It shows that in some sparse high-dimensional settings similar performance as the jointIDA estimators can be obtained, even without estimating the parent sets.

Next, we slightly change our scheme of generating random DAGs to increase the number of confounding paths. We call this "Scheme 2". We ran-

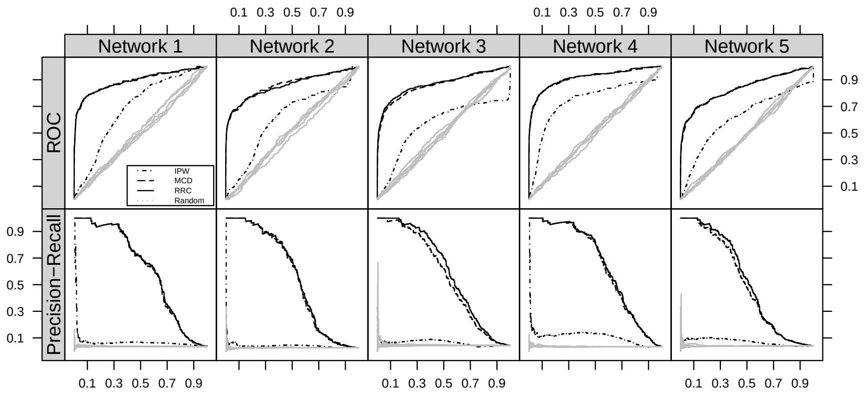


Fig 15: ROC curves (upper panel) and Precision-Recall curves (lower panel) for estimating the target set with top $r$ triples according to the large $|\mathrm{aver}(\bar{\Theta}_{ik}^{(i,j)})|$ values, when the DAGs are generated according to Scheme 1. (Simulated data.)

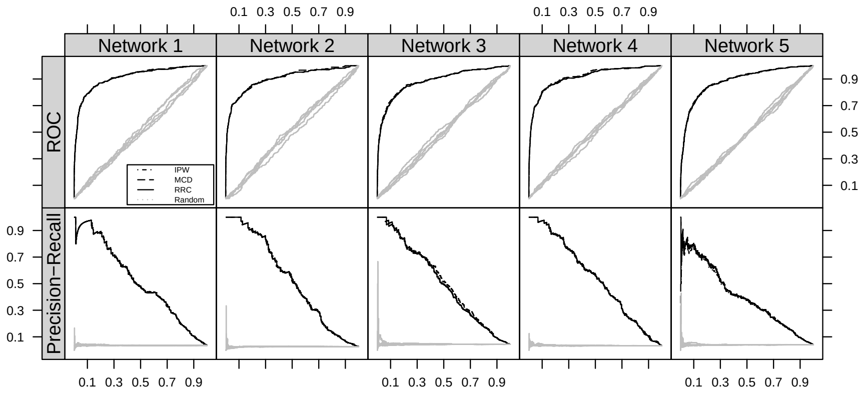


Fig 16: ROC curves (upper panel) and Precision-Recall curves (lower panel) for estimating the target set with top $r$ triples according to the large $|\mathrm{aver}(\bar{\Theta}_{ik}^{(i,j)})|$ values, when assuming that the intervention variables have no parents and the DAGs are generated according to Scheme 1. (Simulated data.)

domly generate a DAG with $p$ vertices and expected neighborhood size $ens$

as follows. We start with an empty DAG with $p$ vertices. Then we choose $\text{Bin}(p, q_1)$ vertices randomly from the vertex set $\{1, \ldots, p\}$ and denote them by $i_1 < \cdots < i_{p^*}$. For each $r \in \{1, \ldots, p^*\}$, we select $\text{Bin}(p - i_r, q_2)$ vertices from the set $\{i_r + 1, \ldots, p\}$ and add an directed edge from $i_r$ to each selected vertex. For given $0 < q_1 \leq 1$, we choose $q_2 = ens/((p-1)\ q_1)$ to ensure that the expected neighborhood size is equal to $ens$.

Note that Scheme 1 is identical to Scheme 2 when $q_1 = 1$, while smaller values of $q_1$ lead to so-called hub-structures, which are common in many biological networks [1]. Figure 17 shows degree distributions of randomly generated DAGs under Scheme 2 for different values of $q_1$.

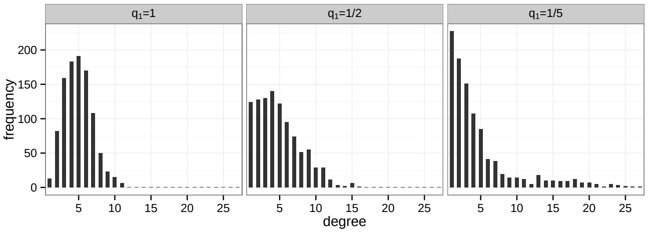


Fig 17: Degree distributions of three randomly generated DAGs under Scheme 2 with $q_1 = 1,\ 1/2$ and $1/5$.

We generate DAGs under Scheme 2 with $q_1 = 1/5$ and construct ROC and Precision-Recall curves as before (Figures 18 and 19). We see that in this case, the joint-IDA estimators based on RRC and MCD outperform the corresponding naive estimators that use empty parent sets. The difference is more apparent in the Precision-Recall curves.

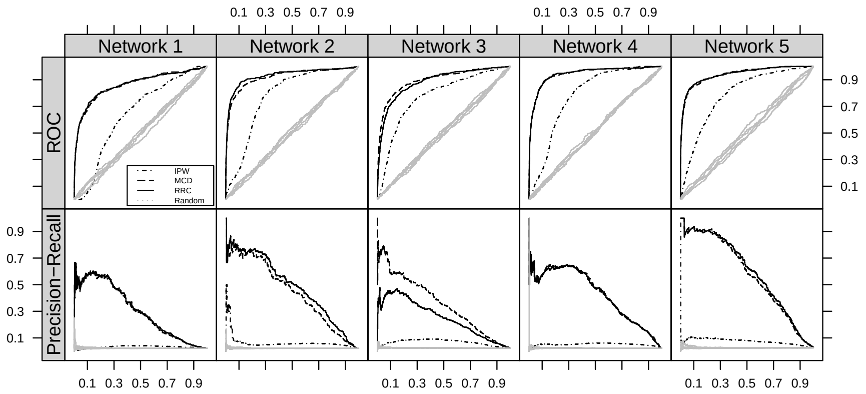


Fig 18: ROC curves (upper panel) and Precision-Recall curves (lower panel) for estimating the target set with top $r$ triples according to the large $|\text{aver}(\bar{\Theta}_{ik}^{(i,j)})|$ values, when the DAGs are generated according to Scheme 2. (Simulated data.)

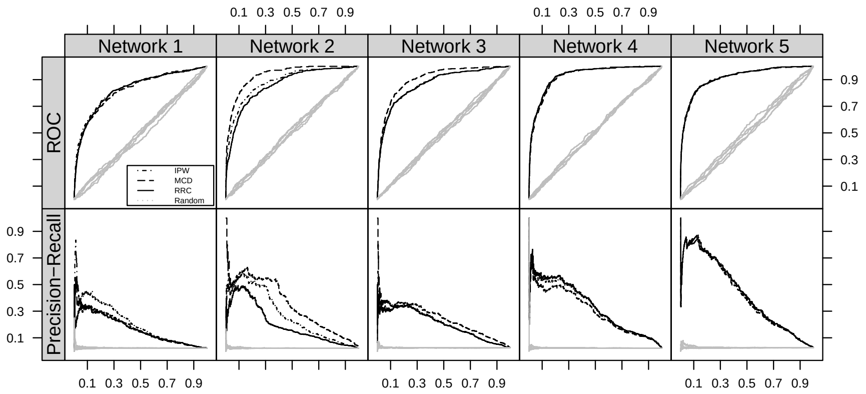


Fig 19: ROC curves (upper panel) and Precision-Recall curves (lower panel) for estimating the target set with top $r$ triples according to the large $|\text{aver}(\bar{\Theta}_{ik}^{(i,j)})|$ values, when assuming that the intervention variables have no parents and the DAGs are generated according to Scheme 2. (Simulated data.)

## 21. Proof of Theorem 7.1 of the main text.

**Proof of Theorem 7.1 of the main text.** Let $\hat{\rho}^S_{nij}$ and $\hat{\rho}^K_{nij}$ denote Spearman's rank correlation and Kendall's rank correlation respectively, between $X_{ni}$ and $X_{nj}$ based on $n$ i.i.d. observations of $\mathbf{X} = \{X_{n1}, \ldots, X_{np_n}\}$. Let $\hat{\Sigma}_{n0}$ be an estimator of $\Sigma_{n0}$, defined as $(\hat{\Sigma}_{n0})_{ij} := 2\sin(\frac{\pi}{6}\hat{\rho}^S_{nij})$ or $(\hat{\Sigma}_{n0})_{ij} := \sin(\frac{\pi}{2}\hat{\rho}^K_{nij})$. Let $||A||_{\max} := \max\limits_{i,j}|A_{ij}|$, for any matrix $A$.

The high-dimensional consistency result of the NPN-joint-IDA estimators follows from high-dimensional consistency of the Rank PC algorithm [6] under the assumptions of Theorem 7.1 of the main text, and the following inequality [6, 10]:

$$\mathbb{P}(||\hat{\Sigma} - \Sigma||_{\max} > \delta) \leq A_1 q_n'^2 \exp(-B_1 n\delta^2), \tag{13}$$

for some constants $A_1, B_1 > 0$, where $\Sigma$ is any $q_n' \times q_n'$ principal submatrix of $\Sigma_{n0}$ with $q_n' = \mathcal{O}(n^{1-b})$ and $\hat{\Sigma}$ is the corresponding principal submatrix of $\hat{\Sigma}_{n0}$. Below, we explain why the arguments given in the proofs of Theorems 6.1 and 6.2 of the main text can be repeated to prove Theorem 7.1 of the main text.

First, recall that in the proof of Theorem 6.2 of the main text, we used the Gaussian assumption only twice, namely (i) for the high-dimensional consistency result of the PC algorithm and (ii) to have the following inequality (see the proof of Lemma 17.3): for any $\delta > 0$, there exists a constant $N > 0$ such that for some $\gamma > 1 - b$ and some constants $A_2, B_2 > 0$

$$\mathbb{P}\left(||\hat{\Sigma} - \Sigma|| > \delta||\Sigma||\right) \leq A_2 \exp\left(-B_2 n^{\gamma}\right) \quad \forall\ n \geq N,$$

for any $q_n' \times q_n'$ principal submatrix $\Sigma$ of $\mathrm{Cov}(\mathbf{X})$ with $q_n' = \mathcal{O}(n^{1-b})$, and for the corresponding submatrix $\hat{\Sigma}$ of the sample covariance matrix.

An analogous inequality can be derived from (13) under the assumptions of Theorem 7.1 of the main text. To this end, note that for any $r \times r$ matrix $A$, $||A|| \leq r\ ||A||_{\max}$. Moreover, since $\Sigma_{n0}$ is a correlation matrix, $||\Sigma|| \geq 1$, for any $q_n' \times q_n'$ principal submatrix $\Sigma$ of $\Sigma_{n0}$. Therefore, from (13), we have,

$$\mathbb{P}\left(||\hat{\Sigma} - \Sigma|| > \delta||\Sigma||\right) \leq \mathbb{P}\left(||\hat{\Sigma} - \Sigma||_{\max} > \delta/q_n'\right) \leq A_1 q_n'^2 \exp\left(-B_1 n\delta^2/q_n'^2\right). \tag{14}$$

Since we assume $2/3 < b \leq 1$ and $q_n' = \mathcal{O}(n^{1-b})$, $\exp\left(-B_1 n\delta^2/q_n'^2\right) \leq \exp\left(-B_3 n^{\gamma}\delta^2\right)$, for some constant $B_3 > 0$ and $\gamma > 1/3 > 1 - b$. This allows us to repeat the rest of the arguments given in the proof of Theorem 6.2 of the main text (see Section 17), to prove the high-dimensional consistency result of the NPN-joint-IDA estimator based on MCD.

Next, recall that the proof of high-dimensional consistency of the joint-IDA estimator based on RRC (Theorem 6.1 of the main text) followed from high-dimensional consistency of the PC algorithm and Lemma 16.1. Analogously, we have high-dimensional consistency of the Rank PC algorithm under the assumptions of Theorem 7.1 of the main text, and below we prove the following inequality (similar to that of Lemma 16.1):

$$\sup_{i<p_n, r\leq m_n} \mathbb{P}(|\hat{\theta}_{ip_n}(\mathcal{G}_{nr}) - \theta_{ip_n}(\mathcal{G}_{nr})| > \delta) \leq A_4 \exp(-B_4\delta^2 n^\gamma), \tag{15}$$

for some constants $A_4, B_4 > 0$ and $\gamma > 1/3 > 1-b$, where $\mathcal{G}_{nr}$ is a DAG in the Markov equivalence class of the true causal DAG, $\theta_{ip_n}(\mathcal{G}_{nr})$ is the total effect of $Z_{ni}$ on $Z_{np_n}$ and $\hat{\theta}_{ip_n}(\mathcal{G}_{nr})$ is the corresponding NPN-RRC estimator.

Note that it is equivalent to prove (15) for the NPN-MCD estimators $\tilde{\theta}_{ip_n}(\mathcal{G}_{nr})$, $i < p_n, r \leq m_n$, since by Theorem 3.5 of the main text, we have, $\tilde{\theta}_{ip_n}(\mathcal{G}_{nr}) = \hat{\theta}_{ip_n}(\mathcal{G}_{nr})$ for all $i < p_n, r \leq m_n$. Thus (15) follows from (14) and from similar arguments that are given in Section 17. □

**22. Simulations in high-dimensional settings under violations of the linearity assumption.** We randomly generate 5 weighted DAGs with $p = 1000$ vertices and expected neighborhood size $ens = 4$, under Scheme 2 with $q_1 = 1/2$ (see Section 20). The edge weights are drawn independently from a Uniform$[0.2, 1.2]$ distribution. We choose two different sets of distributions for the independent error variables: (i) we choose each error variable to be standard normal, and (ii) we randomly choose each error variable to have either a standard normal distribution or a standardized Student's t-distribution with 3 degrees of freedom, each with probability 1/2 (as in Section 20).

For each DAG, we simulate 1000 i.i.d. samples and we transform each data point by taking coordinate-wise cubic transformations, i.e., $\mathbf{g}(x_1, \ldots, x_{1000}) = (x_1^3, \ldots, x_{1000}^3)$. Note that we have data from a nonparanormal distribution in the case where all error variables are Gaussian, but the nonparanormal assumption is violated in the case where some error variables are non-Gaussian.

We randomly choose 20 pairs of intervention variables from each DAG such that no intervention variable is an isolated node in the DAG. For each pair of intervention variables, we choose all other variables that are connected to at least one of the intervention variables by a path (which may or may not be a directed path), as response variables. We choose the target set to be all such ordered triples $(X_i, X_j, X_k)$ for which the total effect of $X_i$ on $X_k$ in the joint intervention on $(X_i, X_j)$ is non-zero (see Section 7 of the main text).

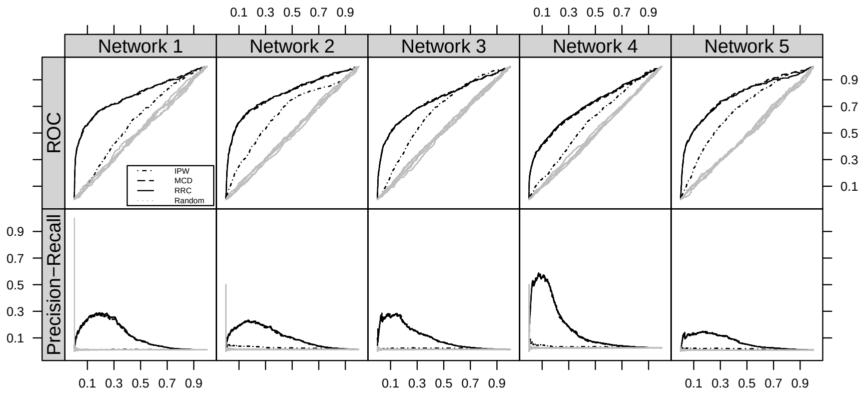


Fig 20: ROC curves (upper panel) and Precision-Recall curves (lower panel) for estimating the target set with top $r$ triples according to the large absolute values of the NPN-joint-IDA estimates based on RRC or MCD, or the joint-IDA estimates based on IPW (after taking the average of each multi-set), when the data are generated from a nonparanormal distribution. (Simulated data, see also Section 7 of the main text.)

We use the NPN-joint-IDA estimators based on RRC and MCD, and the joint-IDA estimator based on IPW (taking the average of each multi-set, as in Section 20) to estimate the target set, where we estimate the underlying CPDAG using an order-independent version of the Rank-PC algorithm [4, 6, 20] with $\alpha = 0.01$.

We construct ROC and Precision-Recall curves for the target set based on the ordered absolute values of the estimates, as in Section 20. Figures 20 and 21 show that the NPN-joint-IDA estimators perform equally well in both settings, and significantly better than random guessing. This suggests insensitivity of the NPN-joint-IDA estimators to slight violations of the nonparanormal assumption in this simulation setting. Poor performance of the joint-IDA estimator based on IPW may be attributed to violation of the linearity and/or the Gaussianity assumption.

Since the NPN-joint-IDA estimators are based on ranks, their performances would remain the same for a different choice of coordinate-wise transformation $\mathbf{g} = (g_1, \ldots, g_p)$, as long as each $g_i$ is a strictly increasing (or strictly decreasing) function. However, the performance of the joint-IDA estimator can be better or worse depending on the transformation.

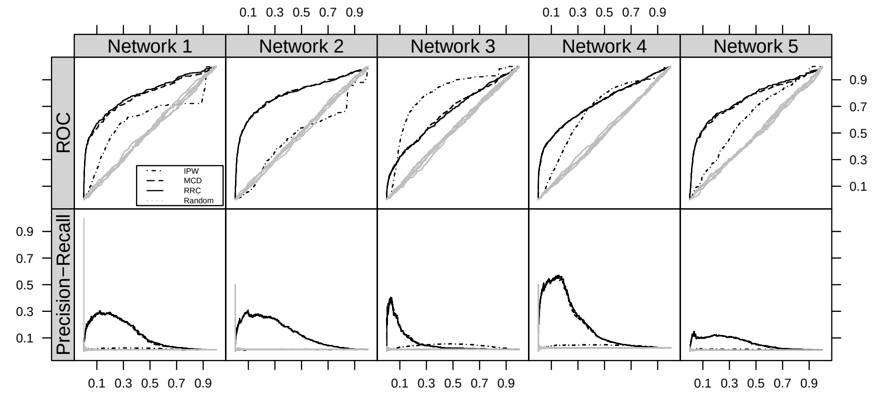


Fig 21: ROC curves (upper panel) and Precision-Recall curves (lower panel) for estimating the target set with top $r$ triples according to the large absolute values of the NPN-joint-IDA estimates based on RRC or MCD, or the joint-IDA estimates based on IPW (after taking the average of each multi-set), when the nonparanormal assumption is violated. (Simulated data, see also Section 7 of the main text.)

**References.**


[1] Albert-Laszlo Barabási and Zoltan N. Oltvai. Network biology: understanding the cell's functional organization. *Nat. Rev. Genet.*, 5:101–113, 2004.

[2] David Maxwell Chickering. Optimal structure identification with greedy search. *J. Mach. Learn. Res.*, 3:507–554, 2002.

[3] W. G. Cochran. The omission or addition of an independent variable in multiple linear regression. *J. R. Statist. Soc. Suppl.*, 5:171–176, 1938.

[4] D. Colombo and M. H. Maathuis. Order-independent constraint-based causal structure learning. *J. Mach. Learn. Res.*, 15:3741–3782, 2014.

[5] Alexander Graham. *Kronecker Products and Matrix Calculus: with Applications.* Ellis Horwood Ltd., Chichester, 1981.

[6] Naftali Harris and Mathias Drton. PC algorithm for nonparanormal graphical models. *J. Mach. Learn. Res.*, 14:3365–3383, 2013.

[7] Lukasz Jasnos and Ryszard Korona. Epistatic buffering of fitness loss in yeast double deletion strains. *Nat. Genet.*, 39(4):550 – 554, 2007.

[8] M. Kalisch and P. Bühlmann. Estimating high-dimensional directed acyclic graphs with the PC-algorithm. *J. Mach. Learn. Res.*, 8:613–636, 2007.

[9] M. Kalisch, M. Mächler, D. Colombo, M.H. Maathuis, and P. Bühlmann. Causal inference using graphical models with the R package pcalg. *J. Statist. Software*, 47(11):1–26, 2012.

[10] Han Liu, Fang Han, Ming Yuan, John Lafferty, and Larry Wasserman. High-dimensional semiparametric gaussian copula graphical models. *Ann. Statist.*, 40:2293–2326, 2012.

[11] M. H. Maathuis, M. Kalisch, and P. Bühlmann. Estimating high-dimensional intervention effects from observational data. *Ann. Statist.*, 37:3133–3164, 2009.

[12] Daniel Marbach, Robert J. Prill, Thomas Schaffter, Claudio Mattiussi, Dario Floreano, and Gustavo Stolovitzky. Revealing strengths and weaknesses of methods for gene network inference. *PNAS*, 107:6286–6291, 2010.

[13] Christopher Meek. Causal inference and causal explanation with background knowledge. In *UAI 1995*, 1995.

[14] P. Nandy, M. H. Maathuis, and T. S. Richardson. Estimating the effect of joint interventions from observational data in sparse high-dimensional settings. 2016.

[15] J. Pearl. *Causality. Models, Reasoning, and Inference*. Cambridge University Press, Cambridge, 2000.

[16] J. Pearl. Causal inference in statistics: An overview. *Stat. Surv.s*, 3:96–146, 2009.

[17] M. Pourahmadi. Joint mean-covariance models with applications to longitudinal data: Unconstrained parameterisation. *Biometrika*, 86:677–690, 1999.

[18] James M. Robins, Miguel Angel Hernan, and Babette Brumback. Marginal structural models and causal inference in epidemiology. *Epidemiology*, 11:550–560, 2000.

[19] Thomas Schaffter, Daniel Marbach, and Dario Floreano. GeneNetWeaver: In silico benchmark generation and performance profiling of network inference methods. *Bioinform.*, 27:2263–2270, 2011.

[20] P. Spirtes, C. Glymour, and R. Scheines. *Causation, Prediction, and Search*. Adaptive Computation and Machine Learning. MIT Press, Cambridge, second edition, 2000.

[21] Ioannis Tsamardinos, Laura E. Brown, and Constantin F. Aliferis. The max-min hill-climbing Bayesian network structure learning algorithm. *Mach. Learn.*, 65(1):31–78, 2006.

[22] Andrea Velenich and Jeff Gore. The strength of genetic interactions scales weakly with mutational effects. *Genome Biol.*, 14(7):R76, 2013.

[23] Thomas Verma and Judea Pearl. Equivalence and synthesis of causal models. In *UAI 1990*, 1990.

[24] R. Vershynin. Introduction to the non-asymptotic analysis of random matrices. In *Compressed Sensing: Theory and Applications*, pages 210–268. Cambridge Univ Press, 2012. Available at http://www-personal.umich.edu/∼romanv/papers/non-asymptotic-rmt-plain.pdf.

[25] Fuzhen Zhang. *The Schur Complement and Its Applications*, volume 4 of *Numerical Methods and Algorithms*. Springer, New York, 2005.

P. Nandy
M. H. Maathuis
ETH Zurich
Seminar for Statistics
Rämistrasse 101
8092 Zurich, Switzerland
E-mail: nandy@stat.math.ethz.ch
E-mail: maathuis@stat.math.ethz.ch

T. S. Richardson
Department of Statistics
University of Washington
Seattle, Washington 98195
USA
E-mail: thomasr@u.washington.edu
